# Supplementary material for: DeepSTORM3D: dense three dimensional localization microscopy and point spread function design by deep learning
Source: arXiv:1906.09957 ancillary file (2019-09-12)
Supplement: Supplementary file 1 [file Supplementary.pdf]

# Supplementary Information

Elias Nehme<sup>1,2</sup>, Daniel Freedman<sup>3</sup>, Racheli Gordon<sup>2</sup>, Boris Ferdman<sup>2,4</sup>, Lucien E. Weiss<sup>2</sup>, Onit Alalouf<sup>2</sup>, Reut Orange<sup>2,4</sup>,  
Tomer Michaeli<sup>1</sup>, and Yoav Shechtman<sup>2,4,\*</sup>

<sup>1</sup>Department of Electrical Engineering, Technion, 32000 Haifa, Israel

<sup>2</sup>Department of Biomedical Engineering & Lorry I. Lokey Center for  
Life Sciences and Engineering, Technion, 32000 Haifa, Israel

<sup>3</sup>Google Research, Haifa, Israel

<sup>4</sup>Russel Berrie Nanotechnology Institute, Technion, 32000 Haifa, Israel

\*Corresponding author: yoavsh@bm.technion.ac.il

## Contents

|                                                |           |
|------------------------------------------------|-----------|
| <b>1 CNN Architectures</b>                     | <b>2</b>  |
| 1.1 Localization CNN                           | 2         |
| 1.2 Optical design CNN                         | 3         |
| <b>2 Physical layer</b>                        | <b>10</b> |
| 2.1 Imaging model                              | 10        |
| 2.2 Poisson noise approximation                | 11        |
| 2.3 Gradient calculation                       | 13        |
| <b>3 Training details</b>                      | <b>15</b> |
| 3.1 Training set                               | 15        |
| 3.2 Loss function                              | 16        |
| 3.3 Optimization and hyper-parameters          | 17        |
| 3.4 Post-processing                            | 17        |
| <b>4 Modified matching pursuit</b>             | <b>17</b> |
| 4.1 Maximum likelihood estimation              | 17        |
| 4.2 Continuous matching pursuit                | 18        |
| <b>5 Assesment metrics</b>                     | <b>19</b> |
| <b>6 Comparison to SMAP-2018</b>               | <b>20</b> |
| <b>7 STORM imaging</b>                         | <b>21</b> |
| 7.1 Phase mask fabrication                     | 21        |
| 7.2 Resolution analysis                        | 21        |
| <b>8 Phase retrieval and wobble correction</b> | <b>22</b> |
| <b>9 Experimental ground truth</b>             | <b>24</b> |
| <b>10 Additional telomere results</b>          | <b>25</b> |

# 1 CNN Architectures

Due to considerations explained later on, we used two different CNN architectures for localizing emitters and for learning a phase mask. First, let us discuss the rationale behind the localization architecture (Fig. S1). As a general rule of thumb, we tried designing simple architectures with the minimal number of parameters needed to solve the problem. Moreover, to handle arbitrary image dimensions we used fully-convolutional CNNs [1]. Furthermore, since the input image contains rich information that needs to be carefully decoded, we passed it via concatenation to all consecutive layers with similar dimensions as an additional feature. To prevent these connections from making the network extremely sensitive to the normalization scheme of the input image, we added a Batch Normalization (BN) layer [2] at the beginning of the architecture that acts as a regularizer and can learn the right normalization of the input image from our training set. To benefit from the input image statistics at test time, we first alter its mean and standard deviation such that it matches the training set statistics:

$$I_{in} = \left( \frac{I_{test} - \mu_{test}}{\sigma_{test}} \right) \times \sigma_{train} + \mu_{train} \quad (1)$$

Where  $\mu_{train}, \mu_{test}, \sigma_{train}, \sigma_{test}$  are the mean and standard deviation of the pixel values of the training set images, and the test image respectively. Then, we feed  $I_{in}$  to the recovery net. While this is a sub-optimal normalization scheme, the resulting architectures were more robust than using an Instance Normalization [3] approach since the test image statistics can vary significantly between experiments. This normalization strategy was particularly useful for the telomere data where the SNR varied significantly between experiments, and was less important for the mitochondria data which exhibited a very similar SNR throughout the STORM experiment. Next, let us discuss the localization architecture in more details.

## 1.1 Localization CNN

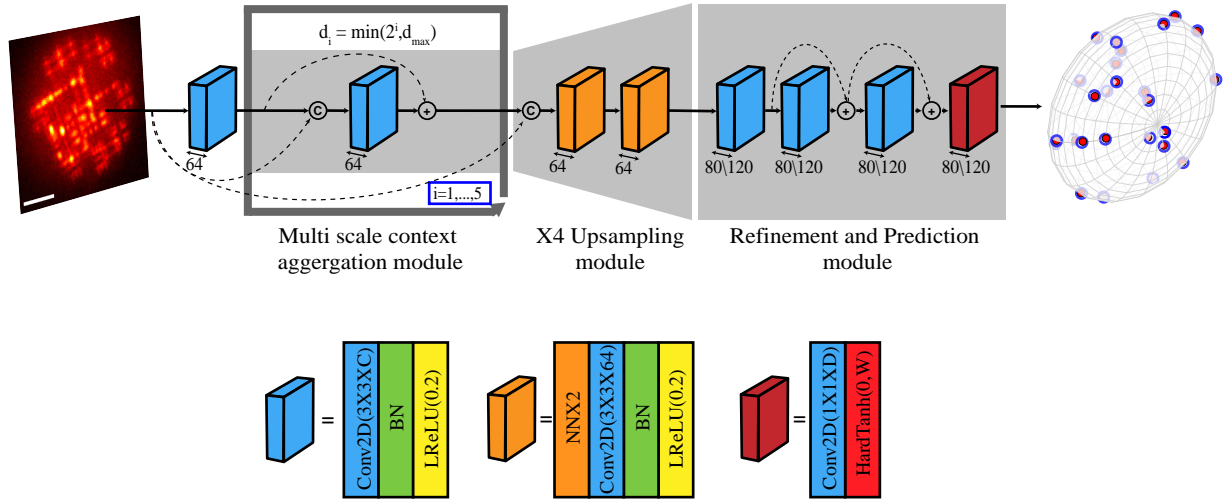

**Fig. S1. Localization architecture.** The low-resolution 2D input image  $I_{in}$  is first passed through a BN layer to normalize pixel values. Next, the normalized image  $I_{norm}$  is passed through the fully convolutional architecture where C denotes concatenation and + denotes element-wise addition. The spatial supports of all convolutional filters are  $3 \times 3$ . The number of channels is fixed to 64 in both the multi-scale context aggregation, and the upsampling modules. Then, the number is increased to 80\120 for the refinement module. The prediction is given by a  $1 \times 1$  convolution followed by a HardTanh activation limiting the range to  $[0, W]$ . The output 3D high-resolution volume is translated to a list of 3D localizations through simple post-processing. An example pair of simulated-input and output are presented before and after the architecture respectively. Blue empty spheres denote simulated positions along the surface of an ellipsoid. Red spheres denote CNN detections. Scale bar is  $3 \mu\text{m}$ .

The proposed architecture (Fig. S1) has only  $\approx 436K \setminus 612K$  trainable parameters and is composed of 3 main modules:

1. Multi-scale context aggregation module: we used dilated convolutions [4] to increase the receptive field of each layer while keeping a fixed number of 64 channels. We set the number of convolution blocks to  $i_{max} = 5$ . The maximal dilation rate  $d_{max}$  was set according to the PSF lateral footprint:  $d_{max} = 16 \setminus 4$  for the Tetrapod and the learned PSF respectively. We also include skip connections to improve gradient flow [5]. Note that this is different from typical architectures used for similar localization tasks in computer vision such as 3D human pose estimation (HPE) [6, 7]. The rationale behind using a simpler architecture with far fewer parameters is that our images have an "easier" context as opposed to extreme semantic variations encountered in HPE.

2. Upsampling module: we used a simple upsampling module composed of two consecutive  $\times 2$  resize-convolutions [8] to increase the lateral resolution by a factor of 4. We used nearest-neighbor interpolation to resize the images. Although more sophisticated upsampling layers with more representation capacity could be used, for example transposed convolution [9–11] or the more recent sub-pixel convolution [12], these layers require a proper initialization to avoid checkerboard artifacts [8, 13] and are not necessary for our task. Assuming a CCD pixel-size of 110 nm, the lateral pixel-size of the upsampled features is 27.5 nm.
3. Refinement module: after super-resolving emitters in the lateral dimension, we further refine their axial position through 3 additional convolutional blocks with an increased number of channels. For a 4  $\mu\text{m}$  range, we use 80/120 channels for the telomere/mitochondria samples respectively, i.e. a voxel-size of 33/50 nm in  $z$ . The final prediction is given by a  $1 \times 1$  convolution followed by an element-wise HardTanh [14] to limit the output range to  $[0, W]$ . As there are only few emitters in a large vacancy volume the classes are highly imbalanced. To take this into account, we weight the ground truth locations by a factor of  $W=800$  determined empirically, and we allow the output of the net to be in the range  $[0, W]$ . This strategy allows us to avoid gradient clipping, and enable meaningful gradients to flow throughout the network during training.

Note that depth is exchanged with channels as our architecture is composed of solely 2D convolutional layers. Afterwards, these dimensions are permuted in the recovered volume. Finally, we threshold voxel-values and find local maxima in clustered components to compile a list of 3D localizations (details in Section 3.4).

In addition, we chose to work with a net that outputs a super-resolved volume (see Section 3.2). However, recovering a vacancy grid is not truly a limitation as it can be combined with a second coordinate-regression net that outputs a continuous list of localizations [15]. Moreover, our recovery voxel-size is either  $27.5 \times 27.5 \times 33 \text{ nm}^3$  or  $27.5 \times 27.5 \times 50 \text{ nm}^3$ , which means assuming the net predicts the right voxel, our precision is limited at worst to  $\approx 20 \text{ nm}$  in the lateral dimension, and  $\approx 17/25 \text{ nm}$  in the axial dimension. This limit is achieved only when encountering an emitter near one of the voxel vertices which is a very unlikely event assuming a uniform distribution. Moreover, as confirmed by our simulations, for images with more than a single emitter the localization precision is not limited by the recovery voxel-size, especially for higher emitter densities.

## 1.2 Optical design CNN

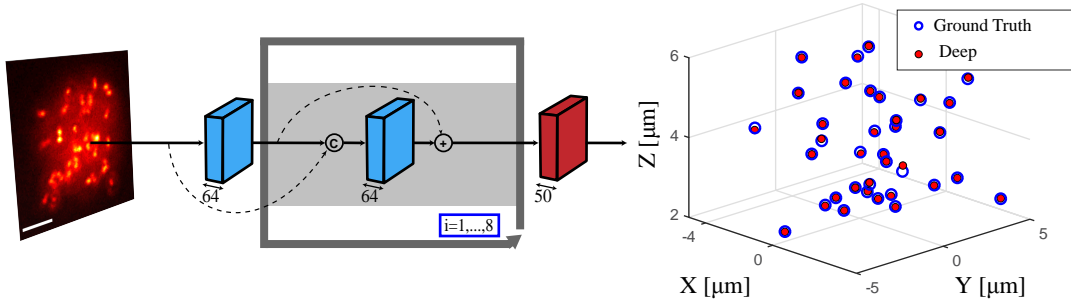

**Fig. S2. Phase mask learning architecture.** The low-resolution 2D input image  $I_{in}$  is first passed through a BN layer to normalize pixel values. Next, the normalized image  $I_{norm}$  is passed through the fully convolutional architecture where C denotes concatenation and + denotes element-wise addition. The spatial supports of all convolutional filters are  $3 \times 3$ . The number of channels is fixed to 64 up until the final prediction where it is reduced to 50. The prediction is given by a  $1 \times 1$  convolution followed by a HardTanh activation limiting the range to  $[0, W]$ . The output 3D high-resolution volume is translated to a list of 3D localizations through simple post-processing. Blue empty spheres denote simulated GT positions. Red spheres denote CNN detections. Scale bar is 3  $\mu\text{m}$ .

Optimally, the architecture used for learning a phase mask should be the same architecture used for localization. Although, calculating the gradients with respect to the phase mask involve computing several FFTs in each forward and backward pass through the net. This added complexity made learning computationally inefficient, and led to inferior results. Hence, to design a phase mask we introduced several modifications to the architecture (Fig. S2). First, the maximal dilation rate was set to  $d_{max} = 1$ , and the number of convolutional blocks was increased to  $i_{max} = 8$ . The receptive field after this modification is  $19 \times 19$ . Next, the upsampling module is eliminated and the lateral dimensions were kept similar to the input CCD image. Finally, the refinement module was also discarded, keeping only the last prediction block (Fig. S1 red block) with a weighting factor of  $W = 100$  and discretization of  $D=50$  in  $z$ , resulting in an  $\approx$ isotropic voxel-size of  $110 \times 110 \times 100 \text{ nm}^3$ . The resulting number of trainable parameters in this modified architecture was only  $\approx 300\text{K}$ .

As was noted in previous work on PSF engineering [16], we empirically observed that it's more efficient to optimize the phase mask with steps of 100 nm in the axial direction (Fig. S4). Moreover, due to refractive index-mismatch, an axial shift of the emitter position is not interchangeable with a shift of the focal plane (see Section 2.1). In the telomere samples we imaged, the emitters were confined to a 4  $\mu\text{m}$  axial range, with the lowest being shifted  $\approx 1 - 3$  microns from the coverslip. To account for the axial range shrinkage, we designed a PSF spanning a larger axial range of  $[0, 5] \mu\text{m}$  with the focal plane centered in 2.5  $\mu\text{m}$ . Finally, as we are first to consider engineering a microscope PSF for high-density localization, we initialized the optimization process with a phase mask implementing zero modulation, meaning, the standard microscope PSF (Fig. 1 main text).

Importantly, in contrast to previous works designing phase masks [16–20], we don’t constrain our design space to be spanned by a fixed set of polynomials (e.g. Gauss-Laguerre modes [17], Zernike modes [16, 19, 20] or concentric rings [18]). Instead, we optimize the phase at each one of the phase mask pixels separately, since this is a much richer class of hypothesis as verified by the learned mask.

Interestingly, learning the phase mask is composed of two main phases; First, the PSF is shaped in the middle  $2\ \mu\text{m}$  range around the focus. Afterwards, once the localization CNN learns to correctly localize emitters in this reduced range, the mask is refined to prevent signal loss at the edges of the axial range and boost the performance at the remaining  $2\ \mu\text{m}$  (see Supplementary Video 1).

Of course, all of the choices above affected the learned phase mask. To study the contribution of the individual choices, we performed the following numerical experiments:

- We learned the phase mask with the localization architecture to study the effect of the net architecture on the result (Fig. S4). Both architectures resulted in extremely similar PSFs regardless of the lateral pixel size in the localization architecture. However, the modified architecture provided denser gradients and distributed the photons more uniformly throughout the axial range.
- We initialized the phase mask to be the Tetrapod mask in order to start from an approximately even distribution of the photons throughout the axial range, and studied the effect of the axial design range and the localization architecture’s receptive field controlled by the maximal dilation rate (Fig. S5). We observed two key results in this experiment. First, with a large enough receptive field ( $d_{\text{max}} = 16$ ) the phase mask is hardly changed regardless of the axial design range. Second, with a smaller receptive field ( $d_{\text{max}} = 4$ ), the resulting PSF had a significantly smaller lateral footprint. This result highlights the importance of the net receptive field when the PSF is initialized to have a large lateral extent. In contrast, when we start from the standard PSF, the receptive field in both cases ( $d_{\text{max}} = 4 \setminus 16$ ) captures the entire initial PSF, and therefore has negligible effect on the learned PSF spatial extent. Moreover, the learned phase mask using the axial range  $[0, 5]$  resulted in a more uniform distribution of the photons throughout the PSF, on the expense of a slight increase in the CRLB.
- The maximal dilation rate was set to  $d_{\text{max}} = 4$ , the axial design range was set to  $[0, 5]$ , and the phase mask was initialized to the double helix (DH) mask [17] (Fig. S6). First, note that the result aligns with the previous experiment emphasizing the fact that when the PSF is initialized to have a smaller lateral footprint than the net receptive field, then it’s hardly modified. This is evident in the result, as the PSF is hardly changed in the middle portion of the axial range. More interestingly, the result suggests that using our method we can extend the DH PSF to a larger axial range of  $4\ \mu\text{m}$  by only modifying it at the edges of the axial range.

Finally, an interesting question arises with respect to the proposed co-design approach. That is, what is the optimal PSF for a single emitter using our method? To answer this question we constrained the number of emitters in each training example to be 1, and set the maximal dilation rate to  $d_{\text{max}} = 16$  in order to enable the learned PSF to have a large spatial footprint (Fig. S7). The axial design range was set to  $[0, 5]$ , and the phase mask was initialized either to the Tetrapod mask or to zero-modulation.

Not surprisingly, when we initialized with the Tetrapod mask, the net hardly changed the phase mask. On the other hand, when we initialized with zero-modulation, the resulting phase mask was extremely different from the phase mask we obtained for the high density case. This time, the net preferred the PSF to have a large spatial extent with "dilated" features in order to ease its localization. Although, when quantifying the localization results for 1000 samples we found the learned PSF to be slightly inferior to the Tetrapod (Fig. S7). This is partially due to our localization architecture being suboptimal for single-emitter localization.

To understand the limit of the achievable performance given our localization architecture, we next calculated the theoretical bound on the RMSE in the lateral and axial dimensions given a voxel-size of  $(\Delta_{xy} \times \Delta_{xy} \times \Delta_z)$ . Assuming emitters are uniformly distributed in each voxel, we can calculate the mean squared error from the middle of the voxel which is the optimal recovered position by the net:

$$\begin{aligned} \text{MSE}_{xy} &= \mathbb{E}_{(X,Y) \sim \mathcal{U}([0, \Delta_{xy}] \times [0, \Delta_{xy}])} \left[ \left( x - \frac{\Delta_{xy}}{2} \right)^2 + \left( y - \frac{\Delta_{xy}}{2} \right)^2 \right] = \frac{\Delta_{xy}^2}{6} \\ \text{MSE}_z &= \mathbb{E}_{Z \sim \mathcal{U}(0, \Delta_z)} \left[ \left( z - \frac{\Delta_z}{2} \right)^2 \right] = \frac{\Delta_z^2}{36} \end{aligned} \quad (2)$$

Substituting our recovery voxel-size of  $(27.5 \times 27.5 \times 50)\ \text{nm}^3$  we get the following lower bounds:

$$\begin{aligned} \text{RMSE}_{xy} &= \sqrt{\frac{\Delta_{xy}^2}{6}} \approx 11\ \text{nm} \\ \text{RMSE}_z &= \sqrt{\frac{\Delta_z^2}{36}} \approx 17\ \text{nm} \end{aligned} \quad (3)$$

Therefore, with the Tetrapod PSF, we are reaching the limit of the achievable precision with our architecture (Fig. S7), and the PSF cannot be improved any further for the single-emitter case. On the other hand, starting from zero-modulation we still have some room for improvement, most likely due to optimization errors. To truly optimize the single emitter case, one needs to consider a different localization architecture that outputs continuous values, which will be addressed in future work.

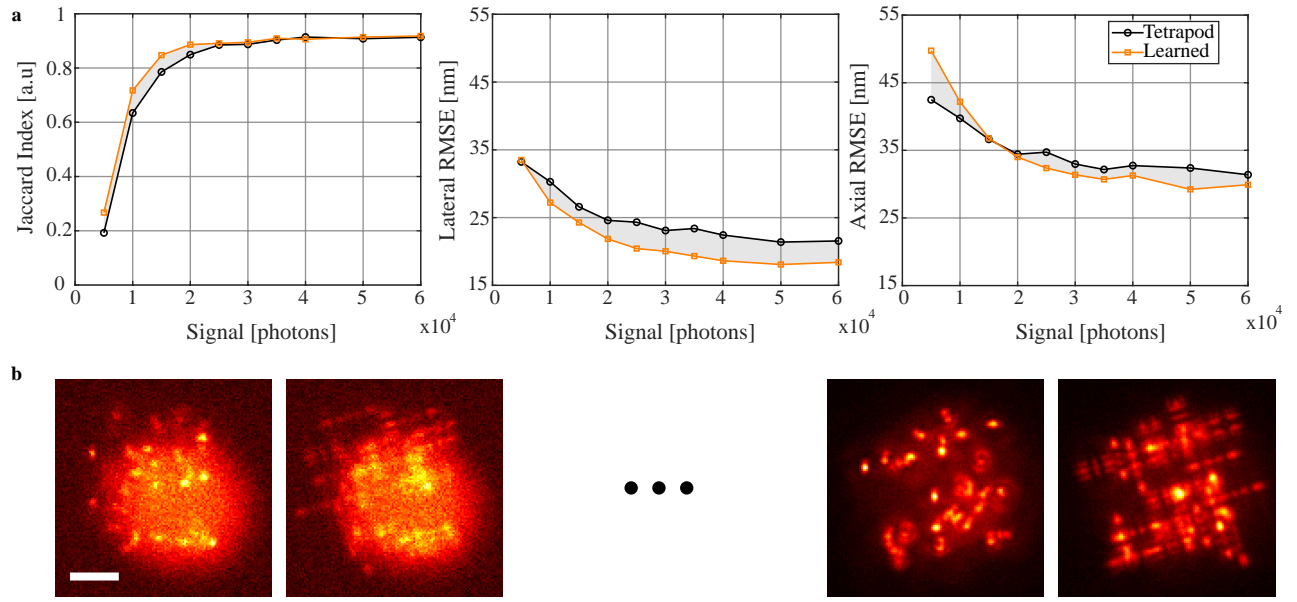

**Fig. S3. Performance as function of SNR.** **a** Comparison of the Jaccard index and the lateral \ axial RMSE as function of signal photons between the Tetrapod-trained CNN (black) and the Learned-PSF CNN (orange) for a fixed density of  $0.124 \left[ \frac{\text{emitters}}{\mu\text{m}^2} \right]$ . **b** Example frames for both PSFs at the lowest (left) and highest (right) tested SNR. Scale bar is 3 μm.

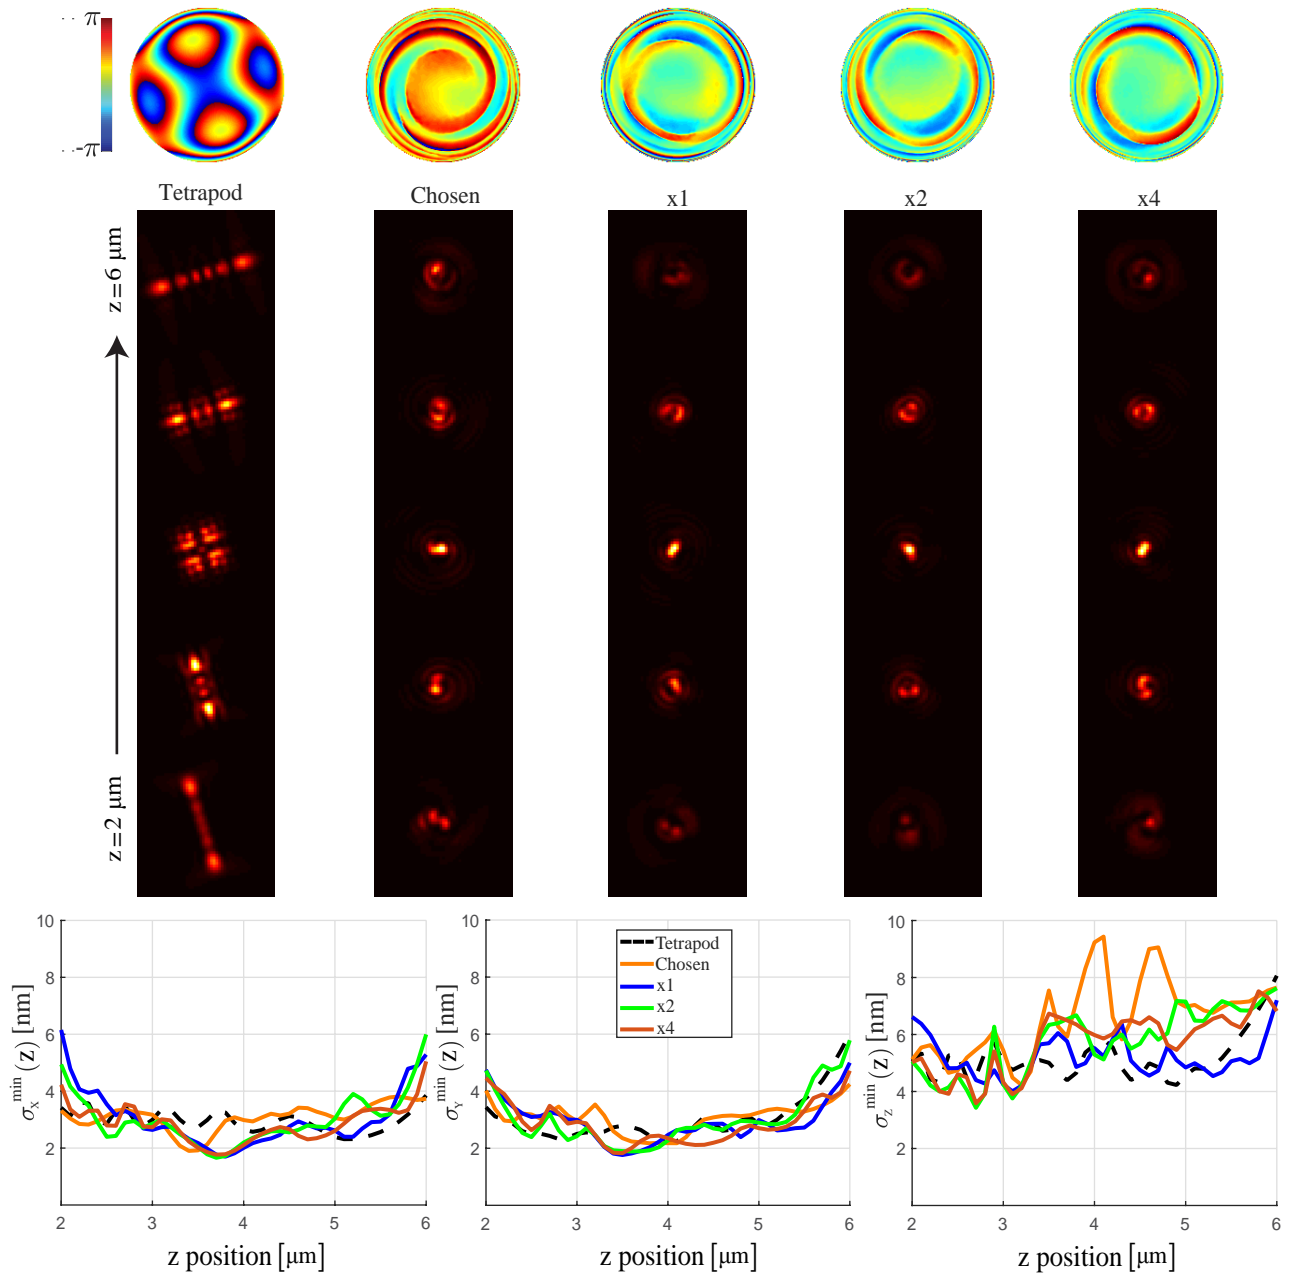

**Fig. S4. Effect of architecture and voxel-size on the learned PSF.** We fixed the optimization and the learning hyper-parameters, set the axial range to  $[2, 6]$ , and learned the phase mask with the localization architecture. To test the effect of the voxel-size in  $xy$ , we tried 3 different settings:  $\times 4$  - the full localization architecture ( $\Delta_{xy} = 27.5$  nm,  $\Delta_z = 50$  nm),  $\times 2$  - the localization architecture with only one upsampling layer ( $\Delta_{xy} = 55$  nm,  $\Delta_z = 50$  nm), and  $\times 1$  - the localization architecture without upsampling ( $\Delta_{xy} = 110$  nm,  $\Delta_z = 50$  nm). The learned masks were similar in all 3 cases. Moreover, compared to the learned mask with the modifications proposed in section 1.2, the resulting PSFs had a lower(better) CRLB on the expense of faster signal loss at the edges of the axial range. The CRLB was calculated assuming 30K signal photons with 160 photons per-pixel background. Similarly to [21] differentiation is done numerically with 1 nm perturbations. Scale bar is  $2 \mu\text{m}$ .

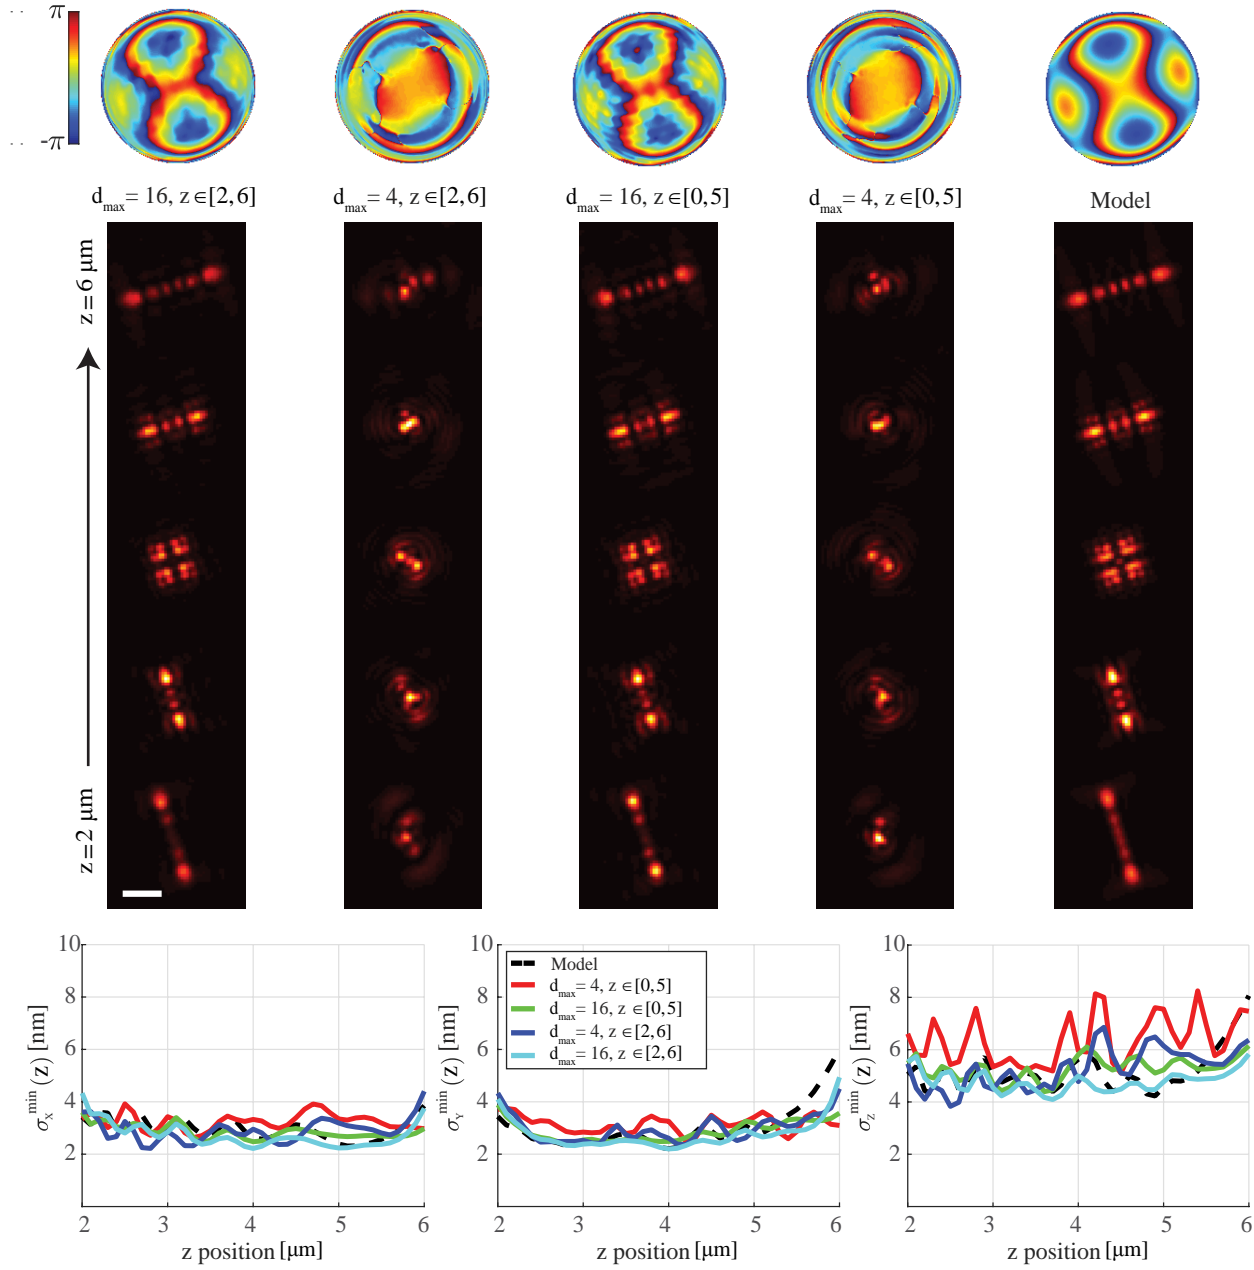

**Fig. S5. Effect of axial design range and the localization net receptive field.** The phase mask was initialized using the Tetrapod model mask (right column), the maximal dilation rate was either  $d_{\max} = 4$  or  $d_{\max} = 16$  corresponding to a receptive field of either  $65 \times 65$  or  $21 \times 21$  pixels, and the axial optimization range was either  $[0, 5]$  or  $[2, 6] \mu\text{m}$ . The larger receptive field resulted in minor modifications to the PSF, while the smaller receptive field enforced it to have a smaller lateral footprint. Moreover, designing the PSF using the larger and lower axial range ( $[0, 5] \mu\text{m}$ ) resulted in a more even distribution of photons on the expense of a slightly increased CRLB. The CRLB was calculated assuming 30K signal photons with 160 photons per-pixel background. Similarly to [21] differentiation is done numerically with 1 nm perturbations. Scale bar is  $2 \mu\text{m}$ .

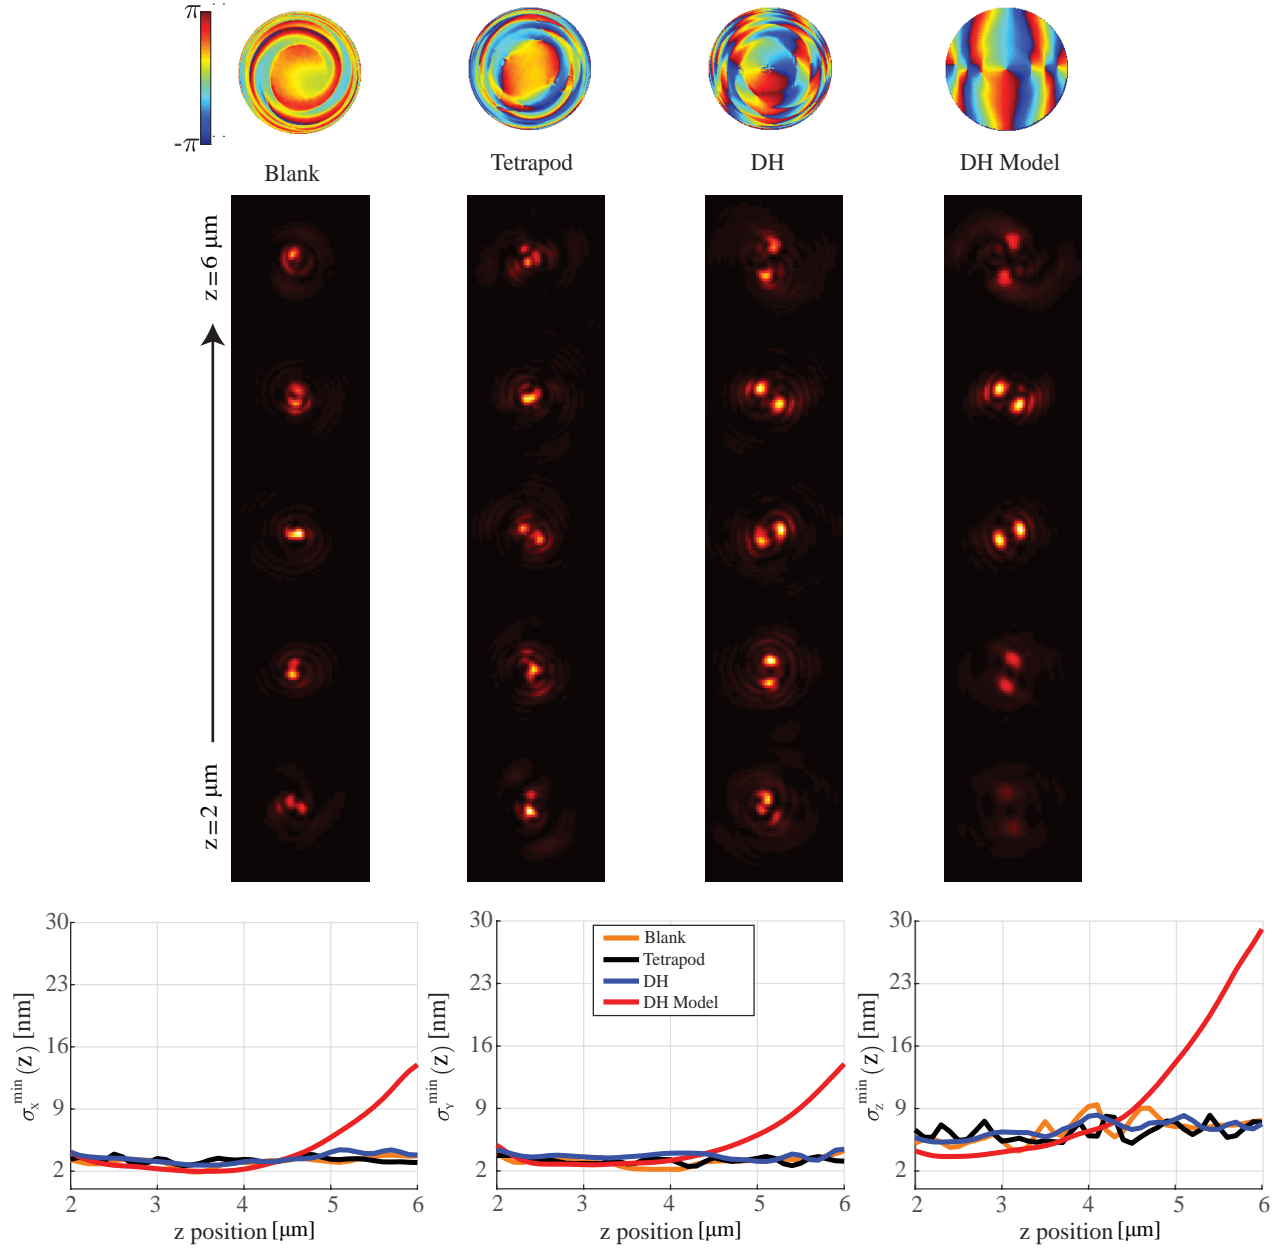

**Fig. S6. Double helix initialization to extend the PSF axial range.** The phase mask was initialized using three different options: (1) Zero-modulation mask, (2) Tetrapod mask, and (3) Double helix mask (right column). The maximal dilation rate was  $d_{max} = 4$ , and the axial design range was  $[0, 5] \mu\text{m}$ . Interestingly, the net didn't modify the double helix PSF in its working range, and only modified it at the edges to capture the full  $4 \mu\text{m}$ . Although compared to the PSF learned with an initial zero-modulation/Tetrapod mask, the double helix initialized PSF was larger, making it potentially harder to localize at extremely high densities. The CRLB was calculated assuming 30K signal photons with 160 photons per-pixel background. Similarly to [21] differentiation is done numerically with 1 nm perturbations. Scale bar is  $2 \mu\text{m}$ .

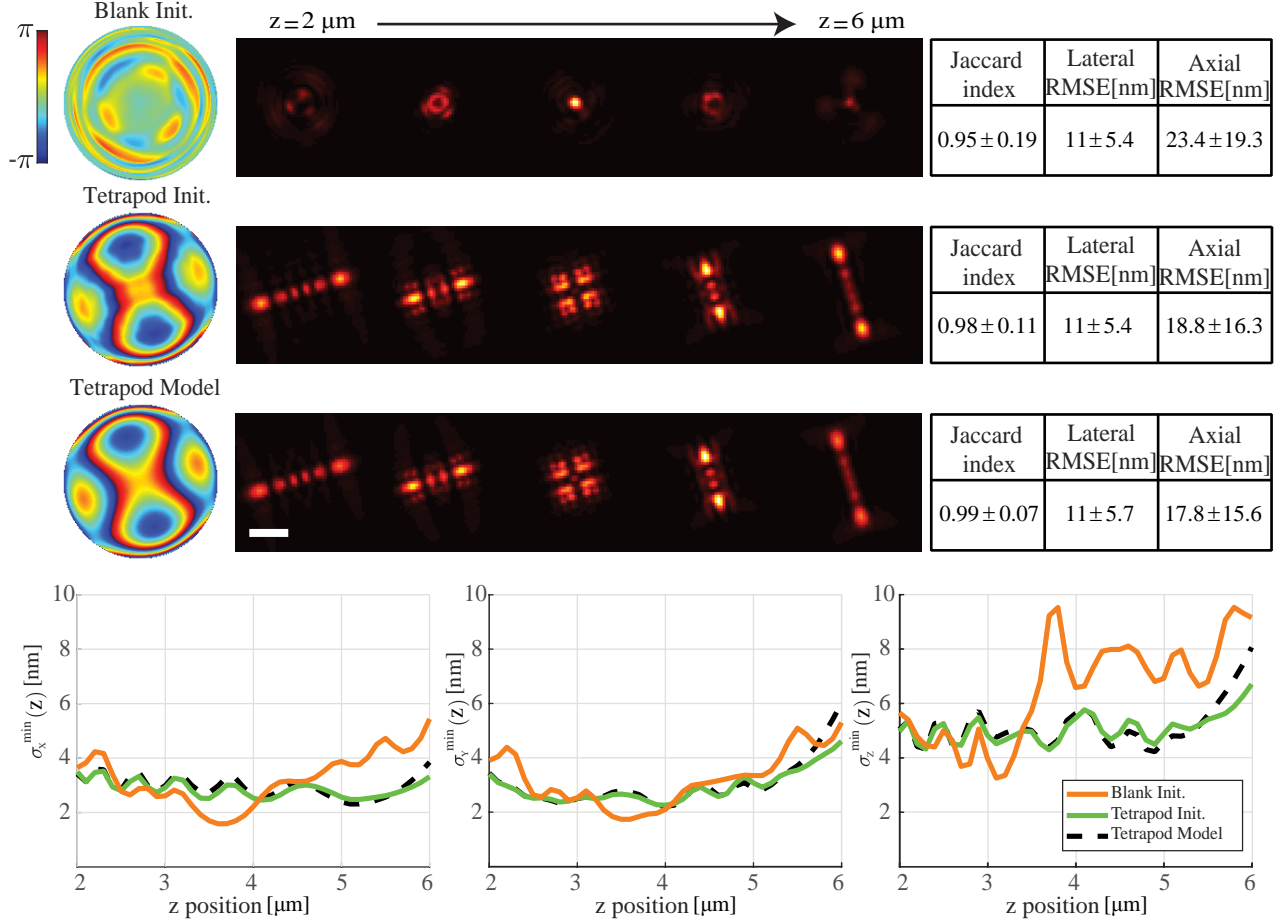

**Fig. S7. Single emitter phase mask learning.** The number of emitters per FOV was dropped to 1. The phase mask was initialized to either blank/zero-modulation, or to the Tetrapod mask. The maximal dilation rate was  $d_{\max} = 16$ , and the axial design range was  $([0, 5] \mu\text{m})$ . The learned PSF for the zero-modulation mask had "dilated" features, while the Tetrapod PSF was hardly changed. Compared to the initial Tetrapod mask, the PSF learned for the blank initialization had slightly worse performance, most likely due to optimization errors. The CRLB was calculated assuming 30K signal photons with 160 photons per-pixel background. Similarly to [21] differentiation is done numerically with 1 nm perturbations. Scale bar is  $2 \mu\text{m}$ .

## 2 Physical layer

### 2.1 Imaging model

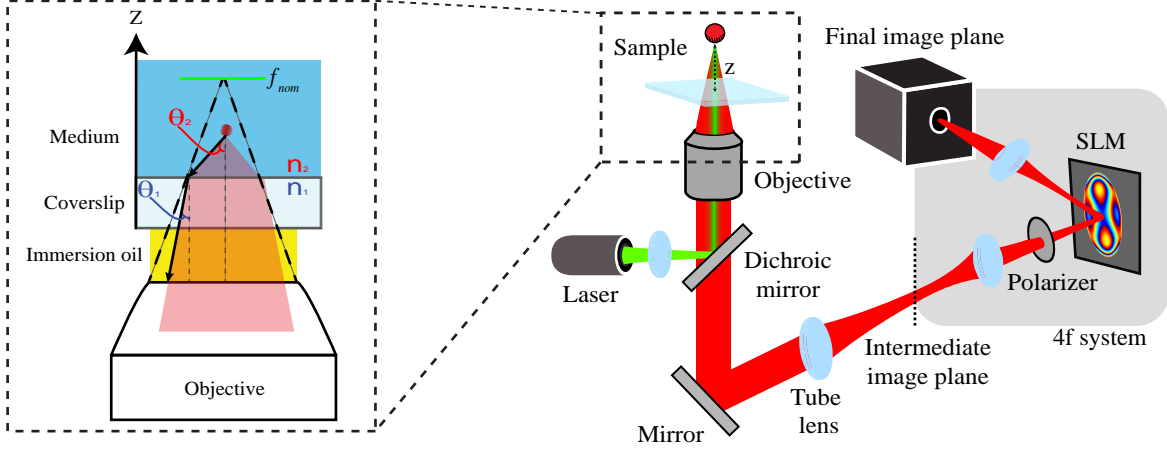

**Fig. S8. Imaging model.** The light emitted from a fluorescent microscopic particle with distance  $z_0$  from the coverslip propagates through the suspension medium (refractive index of water  $n_2 \approx 1.334$ ) with an angle of  $\theta_2$ , and refraction occurs at the interface between the medium and the coverslip. The refracted light propagates in glass/immersion oil (refractive index of  $n_1 \approx 1.517$ ) with an angle  $\theta_1$  and is collected by the objective which is focused at  $f_{nom}$ .

The imaging model used in this work is based on the scalar diffraction approximation of light emitted from an isotropic fluorescent emitter [22]. The optical setup is a 4f-extended microscope with a phase mask implemented by an SLM in the back-focal plane (Fig. S8; reproduced from the main text with additional details for convenience). We assume the emitter is suspended in a medium with a refractive index close to that of water  $n_2 \approx 1.334$ , and is imaged using an oil-immersed objective with a refractive index of  $n_1 \approx 1.517$  matching the glass of the coverslip. Under these assumptions, the PSF in image plane  $I_r(u, v)$  due to a point source located at  $r = (x_0, y_0, z_0)$  is given by:

$$I_r(u, v) \propto |\mathcal{F}_{2D}(E_r(\rho, \phi))|^2 \quad (4)$$

Where  $E_r(\rho, \phi)$  is the electric field at the back focal plane (BFP), and  $\mathcal{F}_{2D}$  denote the two-dimensional Fourier transform. Using Abbe sine rule, the physical dimension of the limiting radius at the BFP due to our 4f-system extension is given by:

$$r_{phys} = \frac{f_{4f} NA}{\sqrt{A_M^2 - NA^2}} \quad (5)$$

Where  $f_{4f}$  is the focal length of each lens in the 4f system, NA is the numerical aperture of the objective, and  $A_M$  is the magnification of the microscope. For convenience, we define two sets of coordinates in the BFP: cartesian  $(\zeta, \eta)$ , and polar  $(\rho, \phi)$ . The polar coordinates are normalized such that  $\rho = 1$  at the limiting aperture given by  $\frac{NA}{n_1}$ . As for the cartesian coordinates, they are given by:

$$\begin{aligned} \zeta &= r_{phys} \rho \cos(\phi) \\ \eta &= r_{phys} \rho \sin(\phi) \end{aligned} \quad (6)$$

The intensity of light is assumed to be uniform within the aperture:

$$circ(\rho) = \begin{cases} 1 & \rho \leq 1 \\ 0 & \text{otherwise} \end{cases} \quad (7)$$

Next, let us derive the terms comprising the phase of  $E_r(\rho, \phi)$ . First, the phase induced by the phase mask  $M$  deployed on the SLM is simply given by the mask itself:

$$\Phi_{mask} = M \quad (8)$$

Let  $\lambda$  denote the emission wavelength,  $k_1 = \frac{2\pi n_1}{\lambda}$  denote the wave-number of the electrical in oil,  $k_2 = \frac{2\pi n_2}{\lambda}$  denote the wave-number of the electrical field in water, and  $f_{nom}$  denote the nominal focal plane. For a point source located above a water-oil interface (Fig. S8) the axial phase is comprised of two parts; First, the axial phase accumulated in water (suspension-medium) due to the emitter distance from the coverslip  $z_0$ :

$$\Phi_{ax_2} = z_0 k_2 \cos \theta_2 \quad (9)$$

Second, the axial phase accumulated in oil due to the focus setting ( $f_{nom}$ ) which is independent of the emitter position:

$$\Phi_{ax_1} = (f_{obj} - f_{nom}) k_1 \cos \theta_1 \quad (10)$$

Where  $f_{obj}$  is the objective focal length. To explicitly calculate the terms in equations (9) and (10), we write Snell's law on the interface:  $n_1 \sin \theta_1 = n_2 \sin \theta_2$ , and use the trigonometric relation  $\cos \theta = \sqrt{1 - \sin^2 \theta}$ . The resulting axial phases are given by:

$$\begin{aligned} \Phi_{ax_1} &= -f_{nom} k_1 \sqrt{1 - \rho^2} \\ \Phi_{ax_2} &= z_0 k_2 \sqrt{1 - \left(\frac{n_1}{n_2} \rho\right)^2} \end{aligned} \quad (11)$$

Where  $f_{obj}$  was dropped since it's already corrected for by the objective. Finally, the lateral shift of the point source ( $x_0, y_0$ ) is modelled using a linear phase:

$$\Phi_{lat} = 2\pi \left( x_0 \frac{\zeta_{AM}}{\lambda f_{4f}} + y_0 \frac{\eta_{AM}}{\lambda f_{4f}} \right) \quad (12)$$

Hence, put equations (8), (11), and (12) together we get the following imaging model:

$$\begin{aligned} I_r(u, v) &\propto \left| \mathcal{F}_{2D} \left( \text{circ}(\rho) e^{j(\Phi_{mask} + \Phi_{ax_2} + \Phi_{ax_1} + \Phi_{lat})} \right) \right|^2 \\ &\propto \left| \mathcal{F}_{2D} \left( \text{circ}(\rho) e^{j \left( M + z_0 k_2 \sqrt{1 - \left(\frac{n_1}{n_2} \rho\right)^2} - f_{nom} k_1 \sqrt{1 - \rho^2} + 2\pi \left( x_0 \frac{\zeta_{AM}}{\lambda f_{4f}} + y_0 \frac{\eta_{AM}}{\lambda f_{4f}} \right) \right)} \right) \right|^2 \end{aligned} \quad (13)$$

To achieve an exact equality the resulting image in equation (13) needs to be rescaled with the amount of signal photons  $N_{photons}$ . In practice, experimental data appears slightly blurred compared to equation (13) due to finite emitter size and aberrations not captured by the model [23]. To remedy this, we blur the result of equation (13) with a small Gaussian filter.

Note that we don't account for dipole effects [21] and instead assume isotropic emission. Moreover, the model disregards the super-critical angle fluorescence (SAF) component which is observed when imaging in small axial ranges ( $< 1 \mu\text{m}$ ) from the coverslip [21, 24]. Finally, we also neglected the intensity apodization factor at the BFP [25]. Nonetheless, since the model was able to describe our experimental data with satisfying accuracy, we made these simplifications to reduce complexity and accelerate our computations.

In contrast to an interpolation-based approach [26–28], a pupil function approach (equation (13)) combined with a phase retrieval procedure [29] is able to accurately model emitters that are distant from the coverslip ( $> \mu\text{m}$ ), potentially alleviating the need for a depth-dependent calibration [30].

## 2.2 Poisson noise approximation

An accurate noise model for an EMCCD camera [27, 31] takes into account three major sources of stochastic noise: shot noise produced by the fluorescence background and signal, Gaussian read out noise produced by the electronics, and electron multiplication noise introduced by the gain process. Our measurements were taken with an sCMOS camera [32] so we didn't include the electron multiplication noise. Assuming we are operating in high photon counts (with no saturation), the readout noise is negligible and the dominant noise source is the Poisson shot noise. In this case, by the law of large numbers, we can approximate the Poisson noise by a Gaussian noise using the central limit theorem:

$$\begin{aligned} y &\approx \text{Poiss}(\lambda = I_{model} + b) \\ &\approx \mathcal{N}(\mu = I_{model} + b, \sigma^2 = I_{model} + b) \end{aligned} \quad (14)$$

Where  $I_{model}$ ,  $b$  are the noiseless model image and the additive background respectively. To enable differentiability of the noise sampling operation, we apply the reparametrization trick [33], and implement the Gaussian noise approximation as:

$$y \approx I_{model} + b + \sqrt{I_{model} + b} \times \epsilon, \quad \text{where } \epsilon \sim \mathcal{N}(0, 1) \quad (15)$$

In the backward pass, the standard noise realization  $\epsilon$  act as a constant, and hence the overall operator is differentiable:

$$\frac{\partial y}{\partial I_{model}} = 1 + \frac{1}{2\sqrt{I_{model} + b}} \times \epsilon \quad (16)$$

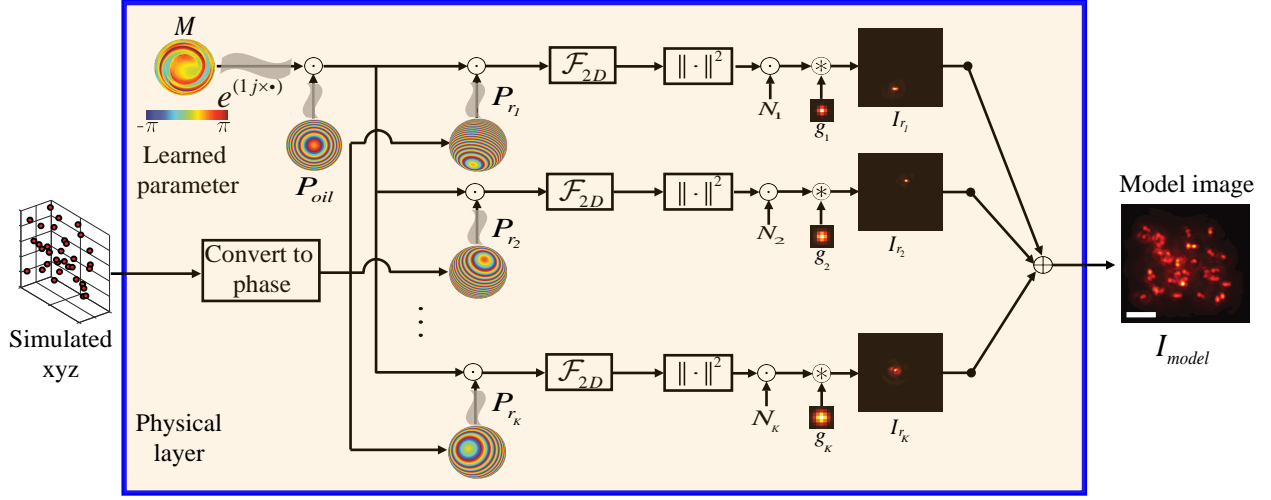

**Fig. S9. Physical simulation layer.** The physical simulation layer is essentially the imaging model in equation (13) viewed as a computational graph, and parametrized by the phase mask. This layer accepts simulated emitter positions as input, calculates an image per emitter, and outputs the 2D model image corresponding to the current mask. The emitters are assumed to be spatially incoherent, hence the output image is given by the incoherent sum of the individual intensity patterns. During training, in each iteration we randomly sample the number of emitters  $K$ , the number of photons per-emitter  $\{N_i\}_{i=1}^K$ , the Gaussian blur per-emitter  $\{g_i\}_{i=1}^K$ , and update the phase mask  $M$  via backpropagation. Scale bar is  $3 \mu\text{m}$ .

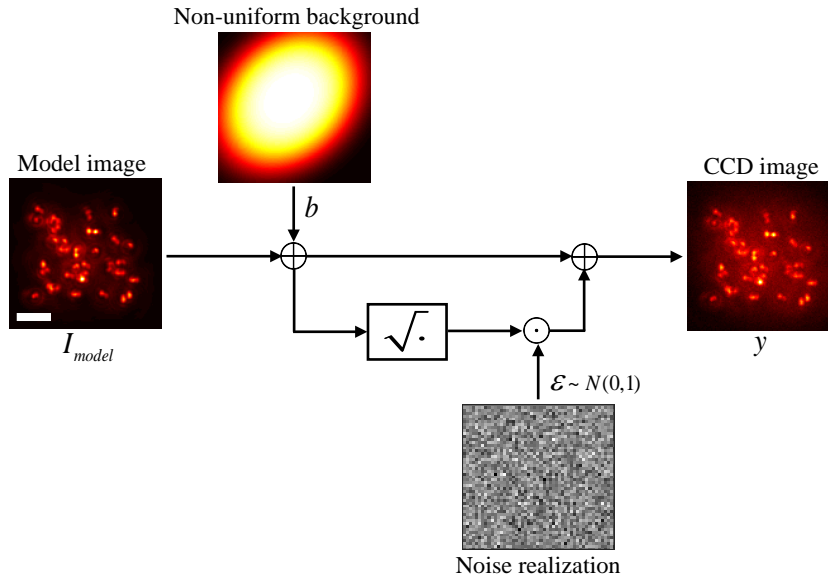

**Fig. S10. Noise approximation.** The mean photons distribution per-pixel is given by the sum of the noiseless model image  $I_{model}$  and the non-uniform background  $b$ . Assuming Poisson statistics This is also the noise variance. Next, to implement a noise variance proportional to the mean, the sum image is passed through an element-wise squared root operation, and multiplied element-wise with a standard Gaussian noise realization. The simulated image on the CCD is modelled by the sum of the mean photons distribution and the noise approximation term. Scale bar is  $3 \mu\text{m}$ .

Of course, our approach is trivially extended with an additive read-out noise realization. In fact, we needed to include this noise source in the training data for the STORM experiment. On the other hand, the telomeres data was shot-noise limited, hence there we didn't bother with this extension. Note that the background term  $b$  is not limited to a constant number of photons per pixel. In fact, to empirically fit our experimental telomeres data we include a non-uniform background (Fig. S10) modelled by a super-Gaussian function:

$$b = A \exp \left( - \left( \alpha_1 (x - x_0)^2 + 2\alpha_2 (x - x_0)(y - y_0) + \alpha_3 (y - y_0)^2 \right)^2 \right) + B \quad (17)$$

With,

$$\alpha_1 = \frac{\cos^2 \theta}{2\sigma_x^2} + \frac{\sin^2 \theta}{2\sigma_y^2}, \quad \alpha_2 = -\frac{\sin 2\theta}{4\sigma_x^2} + \frac{\sin 2\theta}{4\sigma_y^2}, \quad \alpha_3 = \frac{\sin^2 \theta}{2\sigma_x^2} + \frac{\cos^2 \theta}{2\sigma_y^2}$$

Where  $B$  is a baseline value,  $A$  is a normalizing constant,  $(x_0, y_0)$  is the centroid,  $\sigma_x, \sigma_y$  are the on-axis standard deviations, and  $\theta$  is the blob angle. On the other hand, for the STORM experiment we got rid of the non-uniform background by simply subtracting the minimum value per-pixel over the entire acquired stack. This emphasizes an inherent advantage of neural nets over most existing localization methods: tremendous flexibility to cope with a variety of observed challenges.

### 2.3 Gradient calculation

Before we delve into the computation of the gradient, a comment regarding gradients with respect to complex variables is in order. The standard derivative of complex variables is usually studied only for so-called analytical/holomorphic complex functions [34], which have a particular structure in their partial derivatives. Let  $z = x + jy$ , for  $x, y$  real,  $j = \sqrt{-1}$ , denote a complex number and let:

$$f(z) = u(x, y) + jv(x, y) \quad (18)$$

be a general complex-valued function of the complex number  $z$ .  $f(z)$  is said to be holomorphic only if the functions  $u(x, y)$  and  $v(x, y)$  both satisfy Laplace's equation:

$$\frac{\partial^2 u(x, y)}{\partial x^2} + \frac{\partial^2 u(x, y)}{\partial y^2} = 0 \quad \text{and} \quad \frac{\partial^2 v(x, y)}{\partial x^2} + \frac{\partial^2 v(x, y)}{\partial y^2} = 0 \quad (19)$$

Such functions are known as *harmonic* functions. Thus, if either  $u(x, y)$  or  $v(x, y)$  fail to be harmonic, the function  $f(z)$  is not differentiable [34]. However, this class of functions is very limited. For instance, the function  $f(z) = \|z\|^2 = x^2 + y^2$  applied in the physical layer (Fig. S9) is not holomorphic because  $u(x, y) = x^2 + y^2$  is not harmonic. Although, it's clear that  $f(z)$  is a differentiable function of the real and imaginary parts of  $z$ . Hence, an alternative definition of the standard derivative is needed.

For a scalar real-valued function  $\ell$  of a complex-valued variable  $z$ , it's common to define the following gradient [35, 36]:

$$\nabla_\ell(z) = \frac{\partial \ell}{\partial \text{Re}(z)} + j \frac{\partial \ell}{\partial \text{Im}(z)} \quad (20)$$

Moreover, since our graph of mathematical expressions include complex-valued intermediate variables, the usual chain rule cannot be applied. Instead, for  $f(z) = u + jv$  and  $g(z) = r + js$ , the gradient of the real-valued function  $\ell$  with respect to their composition  $f \circ g$  is computed via the "generalized chain rule" (GCR) [35, 36]:

$$\nabla_\ell(g) = \text{Re}(\nabla_\ell(f)) \left( \frac{\partial u}{\partial r} + j \frac{\partial u}{\partial s} \right) + \text{Im}(\nabla_\ell(f)) \left( \frac{\partial v}{\partial r} + j \frac{\partial v}{\partial s} \right) \quad (21)$$

For a thorough and detailed analysis of the complex gradient operator the reader is referred to [37].

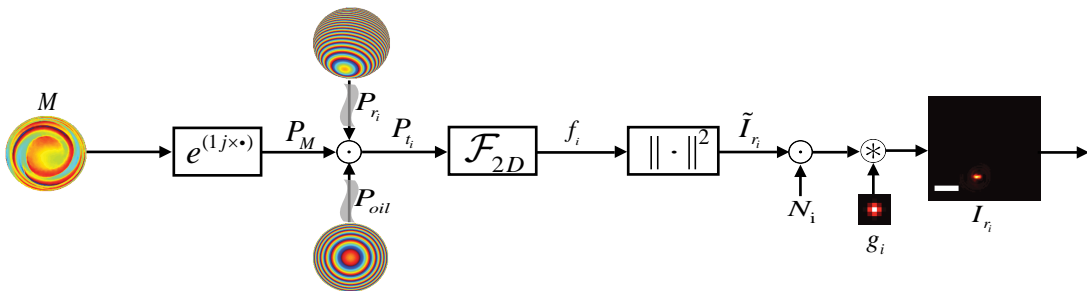

**Fig. S11. Single-emitter image generation pipeline.** The physical simulation layer graph of operations is composed of  $K$  parallel single-emitter image generation pipelines, where the differences between different pipelines are the phase due to the emitter position  $P_{r_i}$ , the number of signal photons  $N_i$ , and the emitter size accounted for by a Gaussian blur  $g_i$ . Scale bar is  $3 \mu\text{m}$ .

Next, to optimize the phase mask in the physical layer (Fig. S9), we need to compute the gradient of our real-valued loss function  $\ell$  with respect to the phase mask. We will not dwell on the gradients of  $\ell$  with respect to the CNN parameters as this is taken care of by the automatic differentiation framework [38]. Instead, we assume we are given the gradient of  $\ell$  with respect to the physical layer output which is the noiseless model image  $I_{model}$  (Fig. S9).

When applying the back-propagation algorithm through a computational graph, a summation is replaced with a fork, and a fork is replaced with summation. Moreover, note that if we shift the global phase term accounting for phase accumulated in oil into each "single-emitter image generation pipeline" (Fig. S11), the gradient back-propagated through each such pipeline will admit a similar expression up to a different position-induced phase term accounting for phase accumulated in water. Hence, for simplicity, we derive the gradient of a single pipeline while keeping in mind that the final gradient will be given by a summation of gradients over all pipelines.

Given the gradient of the loss with respect to the emitter final image  $\frac{\partial \ell}{\partial I_{r_i}} = \frac{\partial \ell}{\partial I_{model}}$ , the gradient  $\frac{\partial \ell}{\partial \tilde{I}_{r_i}}$  is given by:

$$\frac{\partial \ell}{\partial \tilde{I}_{r_i}} = N_i \odot g_i \circledast \frac{\partial \ell}{\partial I_{r_i}} \quad (22)$$

Where  $\circledast$  denotes convolution,  $\odot$  denotes a Hadamard product, and  $g_i$  is not transposed since it's a symmetric Gaussian filter. Next, applying the definition in equation (20) to the relation  $\tilde{I}_{r_i} = \|f_i\|^2$  we get:

$$\begin{aligned} \frac{\partial \tilde{I}_{r_i}}{\partial f_i} &= \frac{\partial \tilde{I}_{r_i}}{\partial \text{Re}(f_i)} + j \times \frac{\partial \tilde{I}_{r_i}}{\partial \text{Im}(f_i)} = \\ &= 2 \text{Re}(f_i) + j \times 2 \text{Im}(f_i) = 2f_i \end{aligned} \quad (23)$$

Furthermore, since the Discrete Fourier Transform (DFT) is a linear operator its gradient is simply the transformation matrix itself. During backpropagation, this gradient is conjugated, hence, by DFT unitarity, this corresponds to the application of the inverse transform [39]:

$$\begin{aligned} \frac{\partial \ell}{\partial P_{t_i}} &= \mathcal{F}_{2D}^{-1} \left\{ \frac{\partial \ell}{\partial \tilde{f}_i} \right\} = \\ &= \mathcal{F}_{2D}^{-1} \left\{ \frac{\partial \ell}{\partial \tilde{I}_{r_i}} \odot \frac{\partial \tilde{I}_{r_i}}{\partial f_i} \right\} = \\ &= \mathcal{F}_{2D}^{-1} \left\{ N_i \odot g_i \circledast \frac{\partial \ell}{\partial I_{r_i}} \odot 2f_i \right\} \end{aligned} \quad (24)$$

Let  $P_{n_i} = P_{r_i} \odot P_{oil}$  denote the combined phase accumulated in water and oil for emitter  $i$ . We apply the definition in equation (21) to compute the gradient with respect to  $P_{M_i}$ :

$$\begin{aligned} \frac{\partial \ell}{\partial P_{M_i}} &= \text{Re} \left( \frac{\partial \ell}{\partial P_{t_i}} \right) \odot \left( \frac{\partial \text{Re}(P_{t_i})}{\partial \text{Re}(P_{M_i})} + j \times \frac{\partial \text{Re}(P_{t_i})}{\partial \text{Im}(P_{M_i})} \right) + \\ &\quad \text{Im} \left( \frac{\partial \ell}{\partial P_{t_i}} \right) \odot \left( \frac{\partial \text{Im}(P_{t_i})}{\partial \text{Re}(P_{M_i})} + j \times \frac{\partial \text{Im}(P_{t_i})}{\partial \text{Im}(P_{M_i})} \right) \end{aligned} \quad (25)$$

Substituting  $P_{t_i} = P_{n_i} \odot P_{M_i}$  in equation (25) we get:

$$\begin{aligned} \frac{\partial \ell}{\partial P_{M_i}} &= \text{Re} \left( \frac{\partial \ell}{\partial P_{t_i}} \right) \odot (\text{Re}(P_{n_i}) - j \times \text{Im}(P_{n_i})) + \\ &\quad \text{Im} \left( \frac{\partial \ell}{\partial P_{t_i}} \right) \odot (\text{Im}(P_{n_i}) + j \times \text{Re}(P_{n_i})) \end{aligned} \quad (26)$$

Once more, we apply the definition in equation (21) again to compute the gradient with respect to  $M_i$ :

$$\frac{\partial \ell}{\partial M_i} = \text{Re} \left( \frac{\partial \ell}{\partial P_{M_i}} \right) \odot (-\sin(M_i)) + \text{Im} \left( \frac{\partial \ell}{\partial P_{M_i}} \right) \odot \cos(M_i) \quad (27)$$

Note that  $M$  is replicated to all pipelines, hence  $M_i = M$ ,  $\forall i \in \{1, \dots, K\}$ . Although, we keep the index  $i$  to denote the gradient of  $\ell$  with respect to  $M$  back-propagated through pipeline  $i$ . Now, recall that a fork in the forward pass of a computational graph is replaced

with summation in the backward pass. Hence, the final gradient with respect to  $M$  is the sum of all gradients  $\frac{\partial \ell}{\partial M_i}$ ,  $\forall i \in \{1, \dots, K\}$ . The steps for calculating  $\frac{\partial \ell}{\partial M}$  are summarized in algorithm 1. This gradient was validated numerically using autograd *gradcheck* function.

---

**Algorithm 1:** Calculation of  $\frac{\partial \ell}{\partial M}$

---

**Input :**  $M, \{P_{n_i}, f_i, g_i, N_i\}_{i=1}^K, \frac{\partial \ell}{\partial I_{model}}$   
**Output:**  $\frac{\partial \ell}{\partial M}$   
**for**  $i \leftarrow 1$  **to**  $K$  **do**  
     $\frac{\partial \ell}{\partial P_{f_i}} \leftarrow \mathcal{F}_{2D}^{-1} \left\{ N_i \odot g_i \otimes \frac{\partial \ell}{\partial I_{model}} \odot 2f_i \right\}$   
     $\frac{\partial \ell}{\partial P_{M_i}} \leftarrow \text{Re} \left( \frac{\partial \ell}{\partial P_{f_i}} \right) \odot (\text{Re}(P_{n_i}) - j \times \text{Im}(P_{n_i})) + \text{Im} \left( \frac{\partial \ell}{\partial P_{f_i}} \right) \odot (\text{Im}(P_{n_i}) + j \times \text{Re}(P_{n_i}))$   
     $\frac{\partial \ell}{\partial M_i} \leftarrow \text{Re} \left( \frac{\partial \ell}{\partial P_{M_i}} \right) \odot (-\sin(M_i)) + \text{Im} \left( \frac{\partial \ell}{\partial P_{M_i}} \right) \odot \cos(M_i)$   
**end**  
**return**  $\frac{\partial \ell}{\partial M} = \sum_{i=1}^K \frac{\partial \ell}{\partial M_i}$

---

### 3 Training details

#### 3.1 Training set

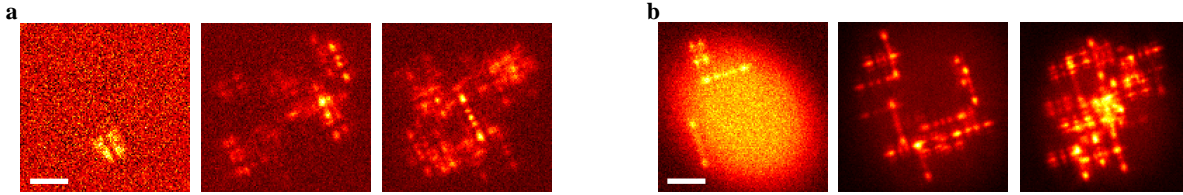

**Fig. S12. Training examples.** **a** The mitochondria training set includes read noise, and signal photons are Gamma distributed. **b** The telomeres training set includes a non-uniform background, and is composed of examples with variable emitter size (blur). Both datasets include variable emitter density and emitter signal-to-noise ratio, with the mitochondria training set (a) having significantly lower SNR. Scale bar is 3  $\mu\text{m}$ .

To learn a localization CNN solely with a predefined phase mask, we simulate a training set composed of 10K simulated images and their corresponding labels which are lists of emitter positions. 9K examples were used for training with 1K examples held out for validation. Alternatively, to jointly learn the phase mask and the localization CNN parameters, the training set is composed of solely simulated emitter positions, as the respective images are being changed throughout iterations according to the phase mask.

Given a set of 3D locations, the expected model image is simulated using a pupil function approach as explained in Section 2. Using a pupil function is preferred over image space interpolation methods as it can accurately capture saddle differences of the PSF. Moreover, from a computational point of view, it's preferred over a convolution followed by a down-sampling approach [27] since we can simulate emitter locations continuously and more efficiently using FFTs. Importantly, while image-space interpolation methods employing splines [26, 28, 40] can capture aberrations which are not well described by a combination of Zernike modes [41], these methods are not suitable for imaging emitters with a large axial shift, as the PSF calibration using beads on a coverslip will not accurately describe the observed PSF due to refractive index mismatch. Therefore, this flexibility in the pupil-function approach is of critical when imaging in cells.

To accurately model experimental data in our simulations we followed the approach of [42] to retrieve the aberrated pupil function for the Tetrapod PSF (see Section 8). As for the designed PSF, we observed that the phase retrieval algorithm failed to recover a reasonable aberration, and hence we generated the training set according to the model pupil function. Interestingly, most of the aberrations in Fourier plane were a result of imperfect implementation of the phase mask on the SLM given a finite set of voltages, rather than misalignment of the optical system, for example. Hence, since the aberration is mask-specific and expected to behave similarly as the implemented phase mask, it's reasonable that it was not well expressed as a linear combination of zernike modes. Although pixel-wise phase retrieval algorithms can be deployed (e.g. [43]), the results with the model were already pleasing, and far better compared to the Tetrapod PSF because of its suitability for high density 3D localization.

To make our simulations more realistic we include experimental variability in our training set. For example, for the telomeres training sets we add a non-uniform background component that is modelled by a super-Gaussian (see Section 2.2) with a randomized angle in the range  $[-\frac{\pi}{4}, \frac{\pi}{4}]$  [rad], randomized standard deviations in the range  $[\frac{\text{FOV}}{5}, \frac{2 \times \text{FOV}}{5}]$  [px], and randomized amplitudes with a baseline value in the range [20, 30] [photons], and a maximal value in the range [120, 180] [photons]. Furthermore, we take into account variations in particle size by convolving each sources' image with a Gaussian blur of a randomized standard deviation in the range [0.75, 1.25] [px] (Fig. S9). Moreover, to enforce robustness to a wide range of conditions, the density of the emitters was varied in

the range  $\left[\frac{1}{\text{FOV}}, \frac{35}{\text{FOV}}\right] \left[\frac{\text{emitters}}{\mu\text{m}^2}\right]$  with a field-of-view (FOV) of  $13 \times 13 \mu\text{m}^2$ . Finally, to prevent the net from over-fitting intensity, the number of signal photons per emitter was varied in the range  $[9\text{K}, 60\text{K}]$  [photons]. Conveniently, the simulated training set can easily incorporate additional experimental challenges such as motion blur, laser fringes, etc. This flexibility is key to making the method versatile and readily extendable for different applications.

In fact, for the STORM experiment, we found that the additive non-uniform background was not necessary since subtracting the minimal value per-pixel of the stack eliminated this issue. However, there we observed a different set of challenges. For instance, while the mean background was relatively constant throughout the FOV, the standard deviation of the read-noise was still higher in the middle of the FOV. Therefore, to take this into account we used the same super-Gaussian from before to scale the standard deviation of the read noise in the range  $[8, 12]$  [photons]. In addition, the number of signal photons per-emitter in the STORM experiment was significantly lower than in the telomeres data, and followed a much less uniform distribution. Therefore, to take this into account we modelled the signal photons in STORM experiment using a Gamma distribution with a shape parameter of  $k = 3000$  [photons] and a scale parameter of  $\theta = 3000$  [photons]. Interestingly, for the STORM experiment, we found it beneficial to alter the GT labels and discard emitters with an extremely low number of photons (below 6K signal photons). This deliberately introduced "label-noise" allowed us to learn a more robust recovery net, coping easily with the non-uniform background introduced by dim/out of range emitters throughout the FOV.

Finally, in our implementation the training set is sampled uniformly within the 3D cube of possible locations. To improve volume coverage, we first sample locations on a coarse grid, and then locally sample a continuous perturbation. Finally, the boolean grid used as a label in training is given by projecting these continuous coordinates using the recovery voxel-size. Although this strategy was simple and convinient in this work, a smarter training set generation can improve learning. For example, a biased sampling scheme with more probability to sample from the edges of the axial range (see Supplementary Video 1) can accelerate convergence, and potentially alter the learned mask, although care must be taken to not introduce artifacts.

### 3.2 Loss function

In computer vision, approaches for inferring the numerical coordinates of key-points in an input image are crudely divided into two classes: approaches that try regressing the coordinates directly using fully-connected (FC) layers (e.g. [26, 44]), and approaches that project the coordinates to the grid using a soft representation (e.g. a heatmap [7, 45]), and afterwards employ representation-matching. The former suffer from two fundamental drawbacks:

1. FC layers limit the model applicability to specific spatial dimensions which necessitates additional manipulation to handle images of general dimensions.
2. FC layers lack inherent spatial generalization [46], which is the ability to generalize knowledge attained at one location during training to another at inference time. This is one of the reasons why augmentation techniques, such as horizontal and axial shifts, are useful for training classification models.

Moreover, a grid representation avoids the inefficient learning of a non-linear mapping from feature space to emitter positions, and provides meaningful voxel-wise supervision. Hence, while FC layers can potentially provide more accurate coordinates, they don't have the generalization ability afforded by spatially shared parameters and are prone to over-fitting [47]. Therefore, we adapt a discrete representation approach, and project the continuous coordinates to the grid.

Next, two alternative approaches can be considered to tackle the task of localization using a CNN. Namely, one approach is to think of localization as a binary classification problem where the CNN predicts a binary occupancy volume, such that 0 denotes an empty/vacant voxel and 1 denotes an occupied voxel containing an emitter. A widely used loss function in this case is the cross-entropy (CE) loss. Although, even for dense localization, the vacant and occupied voxels are highly imbalanced, with only few voxels containing emitters. Therefore, the CE loss is usually either weighted [48], replaced with a Focal loss [49], or applied to a "blobbed" version of the desired boolean volume e.g. by placing a disk around each GT position [50–52]. Afterwards in post-processing, the CNN prediction is usually thresholded, and the final prediction is given by a centroid/local-maximum operation. Alternatively, a second approach is to consider a soft version of the binary classification problem and take a regression route. Namely, by placing a small Gaussian around each GT position (e.g. with std of 1 voxel), we can match continuous heatmaps via an  $\ell_2$  loss [6, 7]. Heatmap matching usually provides more meaningful gradients and ease the learning process convergence. Here, our loss function  $\ell$  is a combination of two terms:

$$\ell(y, \hat{y}) = \|y \otimes g_{3D} - \hat{y} \otimes g_{3D}\|^2 + \lambda \left( 1 - 2 \times \frac{\sum_{i=1}^N y_i \hat{y}_i}{\sum_{i=1}^N y_i + \sum_{i=1}^N \hat{y}_i} \right) \quad (28)$$

Where  $y, \hat{y}$  are the ground truth (GT) and the predicted boolean grid respectively,  $g_{3D}$  is a 3D Gaussian kernel with a standard deviation of 1 voxel,  $\lambda$  is a regularization parameter, and  $N$  is the number of voxels in the prediction grid.

The first term is a heatmap matching term where we measure the proximity of our prediction to the simulated GT by measuring the  $\ell_2$  distance between their respective heatmaps. As for the second term, it is a measure of overlap which provides a soft approximation of the true positive rate in the prediction. Note that this measure doesn't take into account false positives, and hence if optimized alone will result in a predicted volume of 1s. Although, with our loss function this is not a feasible solution as it's not favored by the

first term. The two terms are weighted with a regularization parameter  $\lambda = 1$  determined empirically. In addition, we weight voxels containing emitters with a factor of  $W = 800$  in order to balance out the contributions of vacant and occupied voxels throughout training. Hence, the CNN output is constrained to be in the range  $[0, 800]$ . This strategy makes optimization easier and prevents gradient clipping.

Note that optimally the second term should be replaced with a soft approximation of the Jaccard loss [53] or dice loss [54, 55] which are the metrics we are ultimately interested in optimizing. However, although recent results on approximating the Jaccard loss look promising [56], the high class imbalance between empty and occupied voxels make the optimization process challenging.

To conclude, while the proposed loss function (equation (28)) led to satisfactory results, more optimized choices could further improve performance, for example, a multi-scale approach such as [26]. Alternatively, a non static Gaussian kernel that shrinks over epochs could accelerate convergence. Finally, recent works [46, 57, 58] have suggested bridging the gap between coordinate regression and heatmap matching via the *soft-argmax* function. While in their current version these works assume a known fixed number of key-points and predict a volume per point which is not feasible for localization microscopy, future extensions might prove valuable.

### 3.3 Optimization and hyper-parameters

We used the Adam optimizer [59] with the following parameters:  $\text{lr} = 5 \times 10^{-3}$ ,  $\beta_1 = 0.9$ ,  $\beta_2 = 0.999$ ,  $\epsilon = 10^{-8}$ . The batch size was 16 for learning a phase mask, and 4 for learning a recovery net (due to GPU memory). We experimented with Group Normalization (GN) [60] as an alternative to Batch Normalization (BN) [2] for the smaller batch size, but found that BN gave consistently better results. The learning rate was reduced by a factor of 10 when the loss plateaus for more than 5 epochs, and training was stopped if no improvement was observed for more than 10 epochs, or alternatively a maximum number of 50 epochs was reached. The initial weights were sampled from a uniform distribution on the interval  $[-\sqrt{k}, \sqrt{k}]$  where  $k = \frac{1}{k_x \times k_y \times C_{in}}$ , with  $k_x, k_y$  the filter spatial dimensions, and  $C_{in}$  the number of input channels to the convolutional layer. No further regularization was used (e.g. weight decay [61] or dropout [62]). Training and evaluation were run on a standard workstation equipped with 32 GB of memory, an Intel(R) Core(TM) i7 – 8700, 3.20 GHz CPU, and a NVidia GeForce Titan Xp GPU with 12 GB of video memory. Phase mask learning took  $\approx 25$  h, and recovery net training took  $\approx 35$  h. Our code is implemented using the Pytorch framework [38], and will be made publicly available once this manuscript is accepted for publication.

### 3.4 Post-processing

The final list of localizations is given by the local maximas in the prediction volume that are above a chosen global threshold. While it's possible to use more sophisticated post-processing steps we choose to use this simple and efficient strategy to keep our method as fast as possible. This is extremely important for 3D STORM experiments covering large axial ranges, as these normally entail processing a few tens of thousands of frames. To implement 3D local maxima finding on GPU, we use 3 steps for post-processing:

1. First, the CNN prediction volume is thresholded using the function `torch.where`, with a global threshold normally in the range  $[40, 160]$ . The appropriate choice of the threshold is dependent on the input image Signal-to-Noise Ratio (SNR) and on the accuracy of the PSF model. For example, if the input image has a relatively low SNR (e.g.  $\approx 9K$  signal photons with  $\approx 150$  background photons), or alternatively the training set was generated using the theoretical phase mask rather than a retrieved pupil function, the optimal threshold is more likely to be 40.
2. Second, we discard predictions that are not local maxima in their 3D vicinity. The number of neighboring voxels in the 3D vicinity of the peak was chosen such that the 3D radius for peak finding was  $r_{peak} = 100$  nm for the STORM experiment and  $r_{peak} = 150$  nm for the telomere data. To run this step efficiently on GPU, we compare the thresholded prediction volume to the result of applying the function `torch.nn.MaxPool3d` with a stride of 1 and a kernel size of  $2r_{peak}$  in all three axis. Usually, for a high SNR input image with relatively mild overlaps this step is not necessary. However, This step is crucial for low SNR highly overlapping images, as often the net tends to predict small 3D "blobs" ( $3 \times 3$  cube of values), with the maximum being often in the underlying emitter position. While this step potentially limits the achievable resolution at low SNR, keep in mind that overlaps in 2D normally translates to non-overlapping "blobs" in 3D. Hence, this is merely a limitation for standard imaging experiments using a 2D detector.
3. Finally, we compile a list of localizations by translating the recovered indices to  $\mu\text{ms}$  according to the recovery voxel-size (which is either  $(27.5 \times 27.5 \times 33)$   $\text{nm}^3$  for mitochondria or  $(27.5 \times 27.5 \times 50)$   $\text{nm}^3$  for telomeres).

## 4 Modified matching pursuit

The approach presented below was first described in the supplementary information of [63], and is closely related to [28, 64–66]. Before we go into details, let us first describe the Maximum Likelihood Estimator (MLE) for fitting single emitters which this method builds upon.

### 4.1 Maximum likelihood estimation

MLE is a technique for estimating the parameters of a statistical model based on a set of experimental observations, assuming we know the underlying noise model [67]. Specifically, given the imaging model PSF  $I$  (equation (13)), the Poisson noise model (equation (14)), a measured PSF of a single emitter  $y$ , assuming i.i.d. pixel measurements the likelihood function  $\mathcal{L}$  is given by [68]:

$$\mathcal{L}(\Theta; y) = \prod_{i=1}^M \frac{I_i(\Theta)^{y_i} e^{-I_i}}{y_i!} \quad (29)$$

Where  $\Theta = (x_0, y_0, z_0, N, b)$  is the unknown emitter 3D position and local SNR, and  $M$  is the number of measured pixels. Therefore, the ML estimator is given by:

$$\hat{\Theta} = \underset{\Theta}{\operatorname{argmin}} (-\log(\mathcal{L}(\Theta; y))) \quad (30)$$

$$= \underset{\Theta}{\operatorname{argmin}} \sum_{i=1}^M I_i - y_i \ln(I_i) \quad (31)$$

Where the likelihood maximization problem is exchanged with the equivalent negative log-likelihood minimization problem, and the latter is solved conveniently via MATLAB's `fmincon` routine. This approach is known to achieve results close to the theoretical limit also known as Cramer-Rao Lower Bound (CRLB) [67], and is considered the gold standard for single emitter fitting [68], with available efficient implementations utilizing GPU acceleration [23, 30, 40]. However, for multi-emitter fitting, and specifically for the case of z-dependent PSFs, this approach becomes computationally prohibitive, and alternative approaches need to be explored. An example family of well-performing methods [28, 64–66] are approaches based on "sequential-fitting" as described next.

## 4.2 Continuous matching pursuit

Matching Pursuit (MP) is a method that relies on a sequential fit-and-subtract routine commonly used for sparse signal recovery [69]. Usually, MP is discussed in a discrete setting with a fixed number of possible "atoms" (e.g. PSFs) that can be combined to comprise the measured field-of-view (FOV). Here, we apply a continuous variant of MP, enabled because our dictionary is given by a continuous generative model of the PSF (equation (13)). The basic idea is to decouple the multi-emitter fitting problem into sequential single-emitter fitting sub-problems, where in each iteration we fit the emitter that is most correlated with the residual. Next, the fit result is subtracted and the residual is updated. This process is iterated till a convergence criterion is met.

More formally, first, we start by creating a coarse dictionary  $\mathcal{D}$  with atoms  $a_k$  comprised of the model PSF  $I_r$  (equation (13)) sampled at  $r_k = (x_0 = 0, y_0 = 0, z_0 = k\Delta_z)$ , with  $\Delta_z = 200$  nm,  $k \in \{0, \dots, 20\}$ . The atoms are normalized to have a unit  $\ell_2$  norm:  $a_k^{norm} = \frac{a_k}{\|a_k\|}$ . Second, we set the residual  $R$  to be the measured image  $y$  normalized to have a unit  $\ell_2$  norm:  $R = \frac{y}{\|y\|}$ . Next, we initialize the set of recovered locations  $S$ , and in each iteration we repeat the following steps:

1. Calculate the normalized correlation volume with the residual defined as:

$$N_{corr}[m, n, k] = R[m, n] \otimes a_k^{norm}[-m, -n] \quad \forall k \in \{0, \dots, 20\} \quad (32)$$

2. Find the maximally correlated PSF from the dictionary in the coarse 3D grid:

$$(\hat{m}, \hat{n}, \hat{k}) = \underset{m, n, k}{\operatorname{argmax}} N_{corr}[m, n, k] \quad (33)$$

3. Crop a fixed region from the residual  $R$  around the coarse localization from the previous step:

$$R_c = R[\hat{m} - \Delta_{xy} : \hat{m} + \Delta_{xy}, \hat{n} - \Delta_{xy} : \hat{n} + \Delta_{xy}] \quad \text{with} \quad \Delta_{xy} = 25 \text{ [px]} \quad (34)$$

4. Fit the cropped residual  $R_c$  using MLE (equation (31)) initialized with  $(\hat{m}, \hat{n}, \hat{k})$  to refine the emitter 3D position and estimate the signal and background photons:

$$\hat{\Theta} = (\hat{x}_0, \hat{y}_0, \hat{z}_0, \hat{N}, \hat{b}) = \underset{\Theta}{\operatorname{argmin}} (-\log(\mathcal{L}(\Theta; R_c))) \quad (35)$$

5. Update the set of recovered emitter positions:

$$S = S \cup (\hat{x}_0, \hat{y}_0, \hat{z}_0) \quad (36)$$

6. Calculate the emitter model image  $I_{\text{emitter}}$  using equation (13) with the estimated parameters  $\hat{\Theta}$ :

$$I_{\text{emitter}} = \hat{N} \times \frac{I_{\hat{r}=(\hat{x}_0, \hat{y}_0, \hat{z}_0)}[m, n]}{\sum_m \sum_n I_{\hat{r}}[m, n]} + \hat{b} \quad (37)$$

7. Subtract  $I_{\text{emitter}}$  to update the residual for further fitting:

$$R = R - I_{\text{emitter}} \quad (38)$$

Convergence is achieved when either the mean residual drops below a threshold (e.g. mean background per-pixel), or the overall estimate  $I_S$  correlation with the measured image plateaus.

Note first that the run-time and amount of computations grow linearly with the number of emitters in the field-of-view. Hence, the approach is extremely inefficient for dense fields of overlapping emitters. Second, the strategy taken in step 4 is sub-optimal since the images of overlapping emitters are not explained well by single-emitter fitting. One famous extension of MP is the Orthogonal Matching Pursuit (OMP) method [70] where in each iteration all accumulated emitters in the set  $S$  are re-fitted. In our case this approach is computationally prohibitive, and is not trivially implemented using MATLAB's `fmincon`. Finally, note that for a measured image with a single-emitter, the approach above reduces to single-emitter fitting with MLE, and hence is more accurate than our CNN which is limited by the resolution of the output grid (first data point in Fig. 2 main text). This is because our method was tailored to handle high emitter densities by bounding the precision for the single-emitter case. Although, as shown by recent works [42, 71], CNNs designed specifically for single-emitter fitting can achieve precision comparable to that of MLE. Hence, a cascaded approach combining our method with one of [42, 71] could be considered for further accuracy improvement.

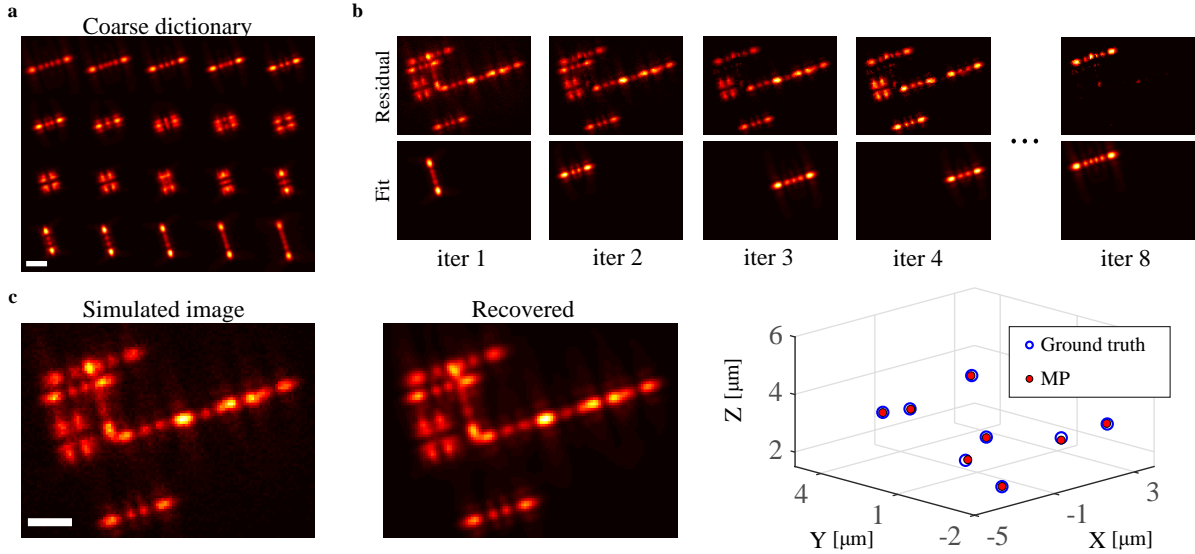

**Fig. S13. Continuous matching pursuit.** **a** Coarse dictionary with 20 atoms  $a_k$  centered in  $xy$  and spaced with 200 nm steps in  $z$ . **b** Example unfolding of the MP iterations (residual - top, fitted emitter image - bottom) for a simulated image with 8 overlapping emitters. **c** Left: Input image is compared with the overall estimated image  $I_S$  by MP. Right: 3D comparison of the simulated emitter positions and the set of recovered positions by MP  $S$ . Scale bar is 3  $\mu\text{m}$ .

## 5 Assessment metrics

To compare localizations directly, we first need to solve the assignment problem [72], meaning, we need to match each recovered position  $(x_i^{\text{rec}}, y_i^{\text{rec}}, z_i^{\text{rec}})$  to a nearby ground truth (GT) position  $(x_j^{\text{gt}}, y_j^{\text{gt}}, z_j^{\text{gt}})$  such that the overall euclidean distance between matched points is minimized. The matching was computed using the Hungarian algorithm [72] with a threshold distance of 150 nm to rule out False Positives (FP). Recovered points that were matched to a GT point were regarded as True Positives (TP). And finally, GT points that were not matched were regarded as False Negatives (FN). Next, following [27] we computed three standard metrics to compare two sets of points:

a. Jaccard Index (JI) defined as:

$$\text{JI} = \frac{\text{TP}}{\text{TP} + \text{FP} + \text{FN}} \quad (39)$$

This metric measures the fraction of correctly identified points in a dataset. A Jaccard index of 1.0 means perfect detection without spurious FPs. It's particularly important for localization techniques to detect a large fraction of the molecules in each frame, as this ultimately dictates the amount of needed frames (e.g. for super-resolution imaging) or more extremely the amount of needed experiment repetitions (e.g. for extracting the diffusion coefficient from single particle tracking trajectories).

b. Root Mean Squared Error (RMSE) in both the lateral ( $xy$ ) and the axial ( $z$ ) dimensions defined as:

$$\text{Lateral RMSE} = \sqrt{\frac{1}{TP} \sum_{i \in S_{TP}} \left( x_{m(i)}^{rec} - x_i^{gt} \right)^2 + \left( y_{m(i)}^{rec} - y_i^{gt} \right)^2} \quad (40)$$

$$\text{Axial RMSE} = \sqrt{\frac{1}{TP} \sum_{i \in S_{TP}} \left( z_{m(i)}^{rec} - z_i^{gt} \right)^2} \quad (41)$$

Where  $m(i)$  is the index of the recovery point matched to GT point  $i$ , and  $S_{TP}$  is the set of matched GT points. These two metrics quantify the precision the localization algorithm, and ultimately determine the achievable resolution. In contrast to the Jaccard index, the RMSE is computed only for TPs and lower is better. Moreover, the lowest achievable precision for an unbiased localization algorithm is bounded by the Cramer-Rao Lower Bound [67].

Although it is possible to define a metric unifying equations (39), (40), and (41) to a single number including also the software runtime [27], throughout this paper we report all 3 metrics separately for convenience.

## 6 Comparison to SMAP-2018

We compared the Tetrapod-trained CNN to SMAP-2018 [40], which is a leading **single-emitter** fitting method that was also successful in localizing high-density of emitters [27]. We ensured that density is the only factor tested by nullifying the effect of SNR, and performing the comparison on a test set composed of Tetrapod PSFs with a high SNR per-emitter.

To use SMAP-2018, we started by calibrating the spline coefficients in order to model the PSF. For this purpose, we simulated an axial stack of a bead PSF covering a  $4 \mu\text{m}$  range with 10 nm steps. The calibration parameters used were the following: ROI size = 41 [px], distance between axial slices = 10 nm, no cross-correlation between slices to for alignment, filter size for peak finding = 8, relative cutoff = 1, smoothing factor = 1. Next, we used the calibrated spline model to localize emitters. For peak finding we used the maximal intensity projection PSF probed at the axial slice  $z = 35$ , with no additional smoothing ( $s = 0$ ). The detection cutoff was set to the absolute (photons) mode with 12 photons, using the maximum criterion. Moreover, we used a rectangular ROI for fitting with 35 [px] sides. MLE fitting was done using the spline model coefficients with 60 iterations of the Levenberg–Marquardt algorithm per emitter. Moreover, for each emitter we initialized the fit with three different starting points in  $z$  ( $z_0 = [-1, 0, 1] \mu\text{m}$ ) and chose the solution with the maximum likelihood. Furthermore, we didn't exclude the rim of the field-of-view (FOV) since some of the PSFs were touching the sides. Finally, to reject false positives and keep only precise localizations, we used the following filtering settings:  $xy\text{-locprec} = 100 \text{ nm}$ , relative Log-likelihood = 2,  $\text{iter} < \text{max}_{\text{iter}}$ , and  $|x_{\text{fit}} - x_{\text{peakfind}}| < 3$ .

Although SMAP-2018 is an excellent single-emitter fitting method, here its performance was worse than MP since it was not designed to handle emitter overlaps. Hence, SMAP being one of the leading software in dense 3D localization for other PSFs [27] highlights the importance of the method presented in this work.

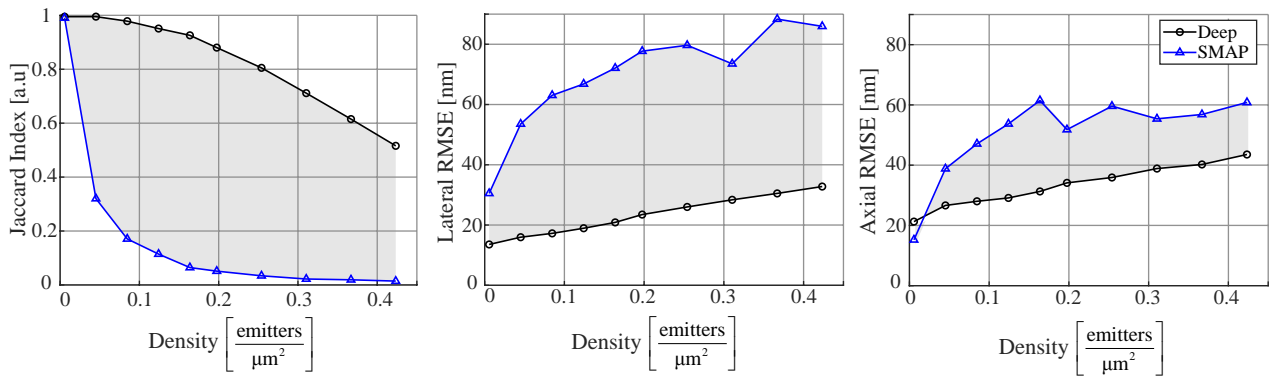

**Fig. S14. Comparison to SMAP-2018.** As expected, the trained CNN is superior to SMAP-2018 in both detectability (Jaccard index) and in accuracy (Lateral \ Axial RMSE). Matching of points was computed with a threshold distance of 150 nm using the Hungarian algorithm [72].

## 7 STORM imaging

### 7.1 Phase mask fabrication

For STORM imaging, the phase mask (PM) was fabricated in fused silica substrate through three iterations of photolithography, with Reactive Ion Etching (RIE) following each step. Chrome-Soda-lime masks were fabricated by a Direct Write Laser Lithography system (Heidelberg DWL66+). The fused silica substrate was coated with positive photoresist Az1518 and baked for 2 minutes at  $90^\circ\text{C}$ , with final thickness of  $2.3\text{ }\mu\text{m}$ . The Karl Suss MA-6 was used as an exposure tool, with an exposure dose of  $28\frac{\text{mJ}}{\text{cm}^2}$  UV light. Three hard mask patterns are prepared, one for each etching step. Next, the wafer was developed in TMAH: DI solution (concentration of 2.25%) for 55 seconds, then rinsed with DI water. After achieving the desired resist pattern, the fused silica wafer was etched by  $\text{CHF}_3$  plasma using a Plasma-Therm 790 RIE. Three steps of photolithography and etching to 140 nm, 280 nm and 560 nm resulted in 8 different heights from 0 to 980 nm, in steps of 140 nm.

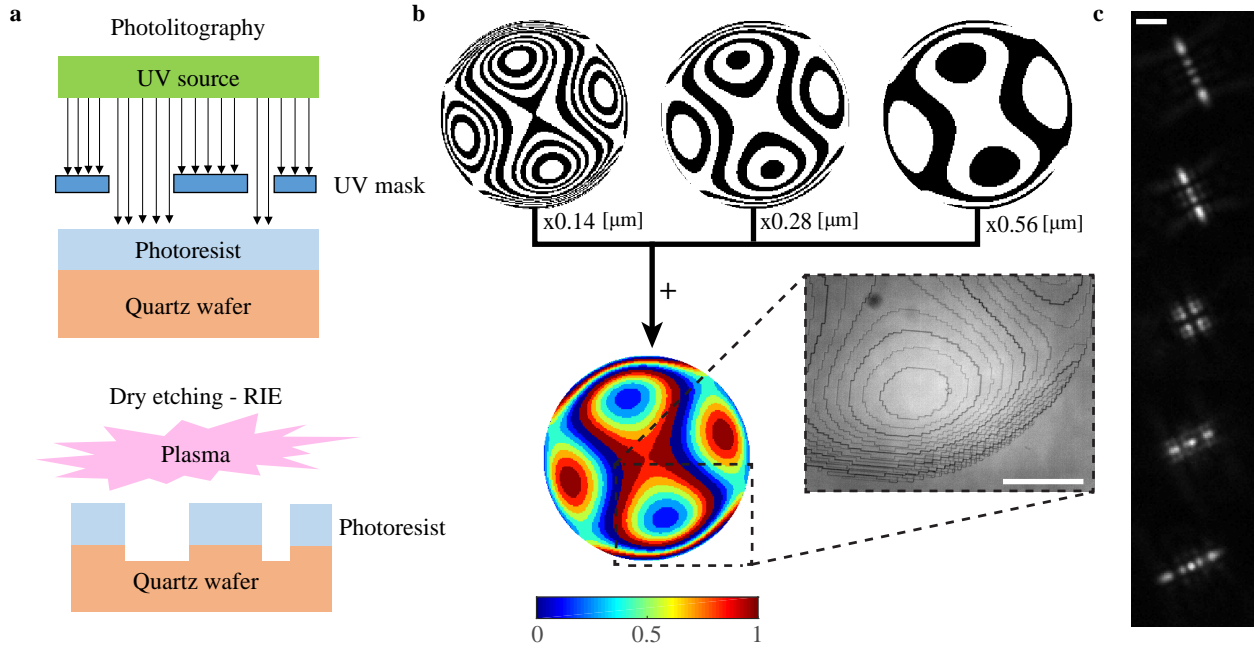

**Fig. S15. Phase mask fabrication.** **a** In the photolithography step (top), a wafer coated with photoresist is illuminated through a hard UV mask. Afterwards, in the dry etching step (bottom), the wafer is etched according to the photoresist pattern. **b** The three UV masks used to generate the 3 corresponding height maps: 140 nm, 280 nm, 560 nm. Since the masks are stacked, the final mask includes 8 different heights, with steps of 140 nm (top). Zoom-in is an experimental measurement of the physical mask using a standard microscope (middle). Scale bar is  $0.5\text{ }\mu\text{m}$ . **c** Measured z-stack of a bead on the coverslip with the physical mask. Scale bar is  $2\text{ }\mu\text{m}$ .

### 7.2 Resolution analysis

To estimate the resolution of our reconstructed super-resolved image, we simulated images with similar SNR using the retrieved phase mask (Fig. S16). The density of the emitters was varied in the range  $\left[\frac{1}{\text{FOV}}, \frac{35}{\text{FOV}}\right] \left[\frac{\text{emitters}}{\mu\text{m}^2}\right]$  with a field-of-view (FOV) of  $13 \times 13\text{ }\mu\text{m}^2$ . To estimate the experimental density we used the number of localizations recovered by the CNN with a low threshold of  $T = 10$ . The resulting density was  $\approx 0.1 \left[\frac{\text{emitters}}{\mu\text{m}^2}\right]$  which means the expected resolution is  $\approx 37\text{ nm}$  in xy and  $\approx 50\text{ nm}$  in z. To compare the result to the single emitter case we calculated the CRLB for a mean signal of  $9000 \left[\frac{\text{photons}}{\text{emitter}}\right]$ , and a mean background of  $140 \left[\frac{\text{photons}}{\text{pixel}}\right]$ . The result suggests that we achieve a factor of  $\approx 2$  relative to the CRLB in precision due to the combination of high density with a low SNR.

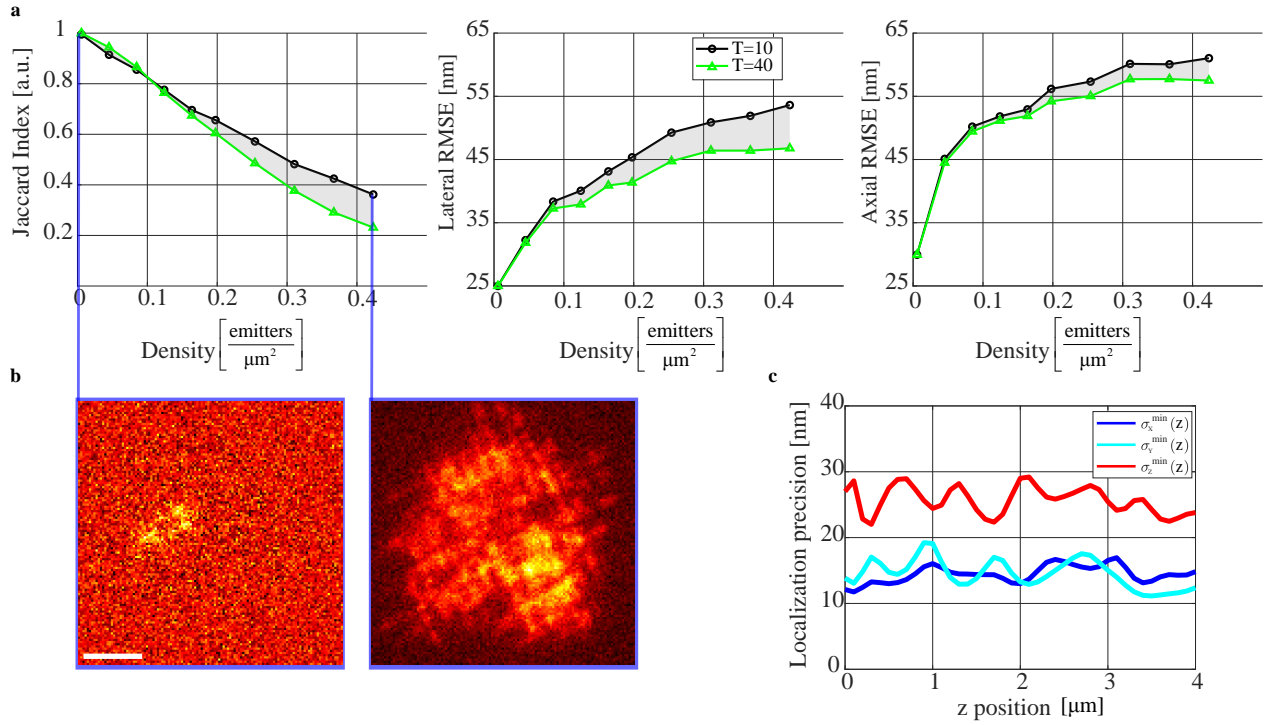

**Fig. S16. STORM resolution analysis.** **a** Jaccard index and Lateral\Axial RMSE calculated at low SNR as a function of density, for two different thresholds  $T = 10\backslash40$ . **b** Example frames with a single emitter (left) and 75 emitters (right). **c** CRLB calculated assuming 9K signal photons with 140 photons per-pixel background. Similarly to [21] differentiation is done numerically with 1 nm perturbations. Scale bar is 3  $\mu\text{m}$ .

## 8 Phase retrieval and wobble correction

An accurate PSF model is crucial to achieve optimal localization precision. Hence, to correct for optical aberrations we implemented a Phase Retrieval (PR) algorithm similar to [29, 42]. First, we scanned the objective with 80 nm steps to acquire an axial stack  $\{y_{f_{nom}^i}\}_{i=1}^{80}$  of a single bead (Tetraspeck 0.2μm) using the same optical setup of the biological experiments, i.e. excited by a 561 nm laser (Toptica iChrome MLE), filtered (Chroma 575/90 bandpass) to have a similar wavelength to the cell experiments.

Note that since the bead is imaged on the coverslip, the imaging model discussed in section 2.1 is not a perfect representation. This is because, near the coverslip (e.g.  $< 1 \mu\text{m}$ ) we need to account for super-critical angle fluorescence which the mask wasn't designed for. Therefore, to nullify this model mismatch from the PR process, and exclusively capture optical aberrations that will be present deeper in the sample, we used a vectorial diffraction model that assumes freely rotating dipoles [21].

The axial position of the bead was fixed to 0.1  $\mu\text{m}$  which is the bead radius. To calibrate the wobble as function of the axial position, we define the centroid of the axial slice matching the focus setting  $f_{nom} = 0$  to be the origin  $(x_0, y_0) = (0, 0)$ . Moreover, the additive aberration was assumed to be a combination of the first 50 Zernike polynomials not including piston and tilt:

$$M_{\text{retrieved}} = M_{\text{theory}} + \sum_{j=2}^{50} a_j Z_j \quad (42)$$

This assumption simplifies the optimization process greatly, and reduces it to estimating only 48 Zernike coefficients. On the other hand, this computational relief comes at the cost of modelling capacity since Zernike polynomials are smooth functions and not well fitted to model phase-jumps (Fig. S17 a (right panel)) such as in the learned mask or the double helix mask [17]. Nevertheless, we were able to obtain excellent results with the theoretical learned mask, therefore we used PR only to refine the Tetrapod mask.

Next, let  $M_{\text{retrieved}}$  denote the retrieved phase mask,  $y_{f_{nom}^i}$  denote the PSF image at focus position  $f_{nom}^i$ , and  $(x_i, y_i)$  denote the lateral displacement from the defined origin. The PR algorithm alternates between two steps:

1. Fix the retrieved phase mask  $M_{\text{retrieved}}$ , and use MLE in conjunction with the model (equation (13)) to estimate the focus position  $f_{nom}^i$ , the SNR  $(N_i, b_i)$ , and the wobble  $(x_i, y_i)$  in each axial slice  $y_{f_{nom}^i}$ :

$$\hat{\Theta}_i = \left( \hat{x}_i, \hat{y}_i, \hat{f}_{nom}^i, \hat{N}_i, \hat{b}_i \right) = \underset{\Theta_i}{\operatorname{argmin}} \left( -\log \left( \mathcal{L} \left( \Theta_i; y_{f_{nom}^i} \right) \right) \right) \quad \forall i \in \{1, \dots, 80\} \quad (43)$$

2. Fix  $\{\Theta_i\}_{i=1}^{80}$ , calculate the respective model images  $\{I_{\Theta_i}\}_{i=1}^{80}$ , and update the retrieved phase mask  $M_{\text{retrieved}}$ :

$$\hat{a}_j = \underset{a_j}{\operatorname{argmin}} \sum_{t=1}^T \sum_{s=1}^S \sum_{i=1}^{80} |I_{\Theta_i}[t, s] - y_{\hat{f}_{nom}}[t, s]| \quad \forall j \in \{2, \dots, 50\}$$

$$M_{\text{retrieved}} = M_{\text{theory}} + \sum_{j=2}^{50} \hat{a}_j Z_j \quad (44)$$

The retrieved phase mask  $M_{\text{retrieved}}$  was initialized to the LC-SLM calibrated theoretical mask  $M_{\text{theory}}$ , and  $\{\hat{f}_{nom}^i\}_{i=1}^{80}$  were initialized to the designed scan positions. Note that differently from [42], here we employed this alternation strategy since the result of each step depends on the result of the other. Therefore, for an accurate calibration of the wobble [73] over a large axial range we need to calibrate it using the already retrieved pupil function. Moreover, this approach was more accurate than simply assuming a known focus position from the stage readout. We found that for our setup 2 iterations were enough to achieve convergence.

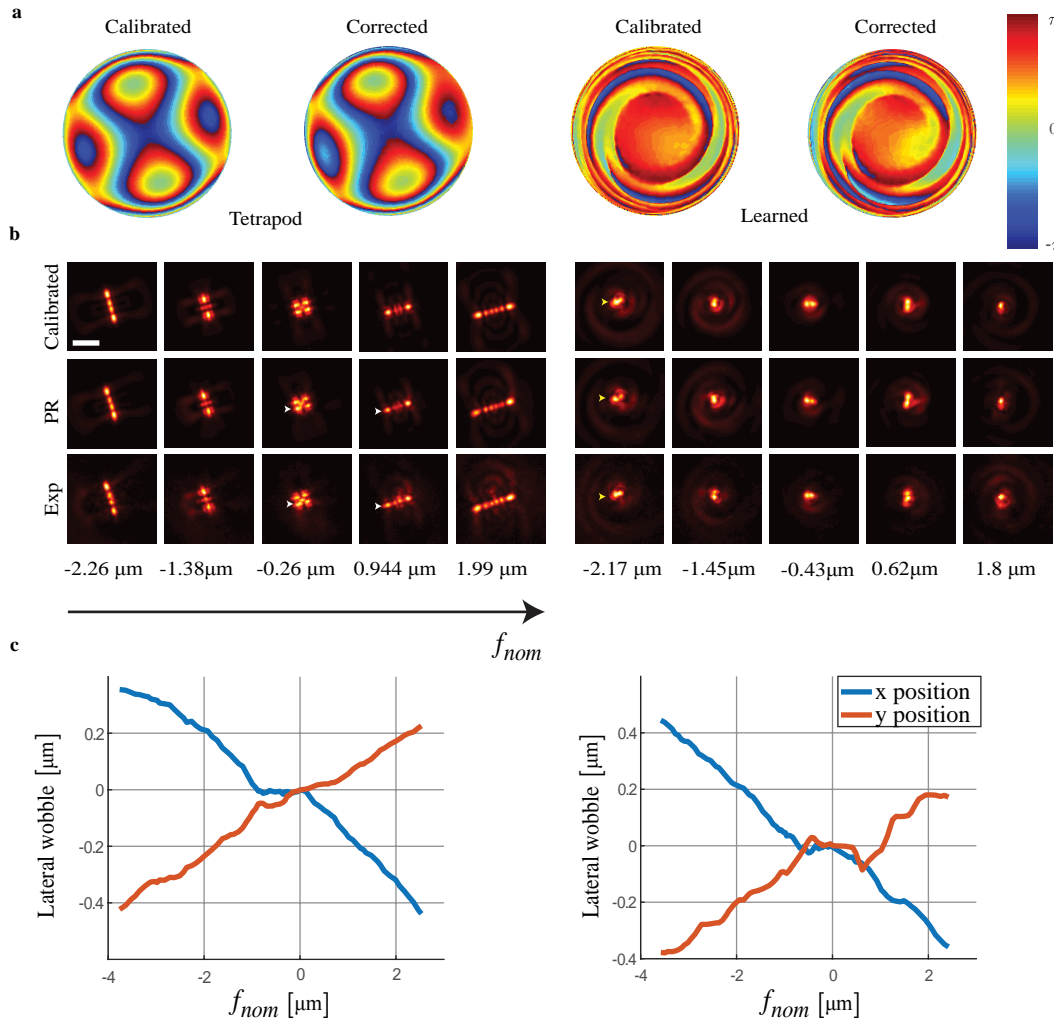

**Fig. S17. Phase retrieval and wobble correction.** **a** Calibrated and retrieved Tetrapod (left) and learned (right) masks. Calibration is achieved by projecting the desired phase pattern on the available LC-SLM calibration voltages. **b** Comparison of the simulated PSFs using the calibrated/retrieved mask to an experimentally measured z-stack of a fluorescent bead with a similar emission wavelength to the cell data. The PR algorithm managed to recover the aberration for the Tetrapod mask (white arrows), and failed to recover it for the learned mask (yellow arrows). **c** Calibrated lateral wobble as function of the focus position for the Tetrapod (left) and the learned mask (right). Scale bar is  $3 \mu\text{m}$ .

## 9 Experimental ground truth

To approximate ground truth 3D positions of the telomeres (Fig. S18), we scanned the sample in the axial direction with 100 nm steps covering a 5  $\mu\text{m}$  range (see Supplementary Data 1). Next, the telomeres were localized in each frame using ThunderSTORM [74] to extract the lateral position (i.e. XY centroid). Afterwards, the approximate axial position of each detected telomere was determined by fitting a 2<sup>nd</sup> order polynomial to the mean intensity profile along 17 adjacent axial slices (Fig. S18 b-d). The resulting z locations were multiplied by a factor of  $\frac{1.33}{1.518}$  to account for refractive index mismatch [75, 76]. To compare the recovered positions to the approximate experimentally calibrated GT, we corrected the lateral recovered position using the wobble calibration matching the recovered axial position. To estimate the wobble for unmeasured axial positions we used cubic spline interpolation.

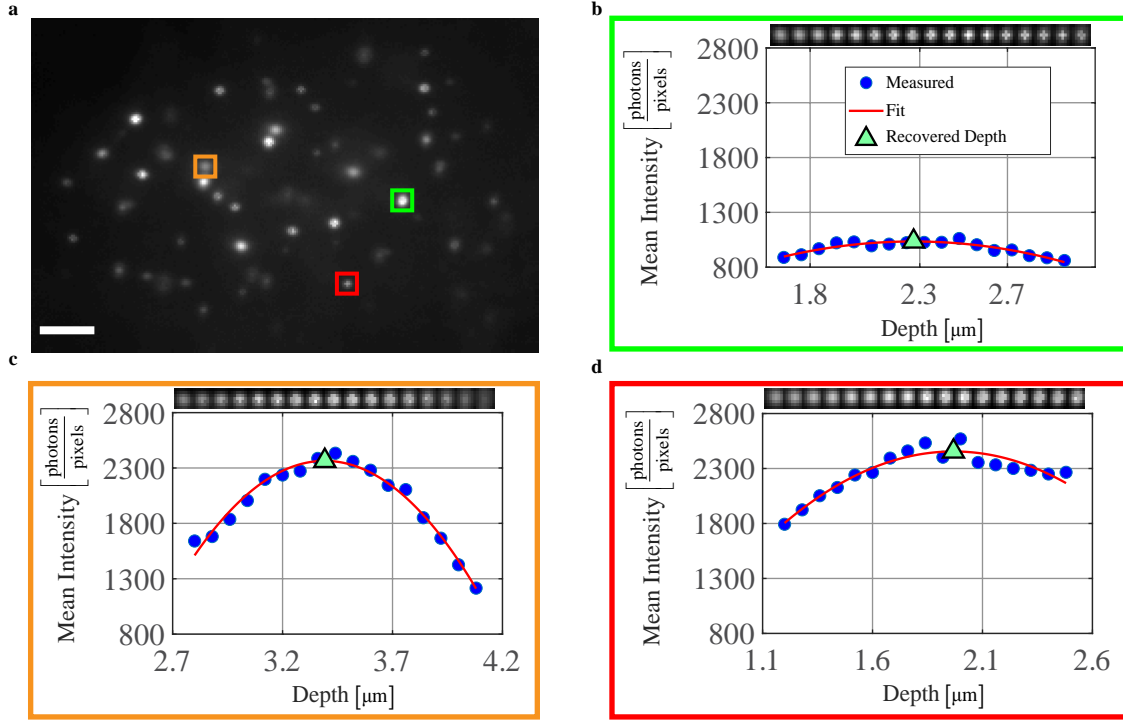

**Fig. S18. Experimental ground truth estimation.** **a** Focus slice with 3 marked emitters. **b - d** Estimation of the axial position for the 3 emitters. The emitters vary in size (e.g. **b** vs. **d**) and signal photons (e.g. **b** vs. **c**), therefore the fit accuracy is limited. Scale bar is 3  $\mu\text{m}$ .

## 10 Additional telomere results

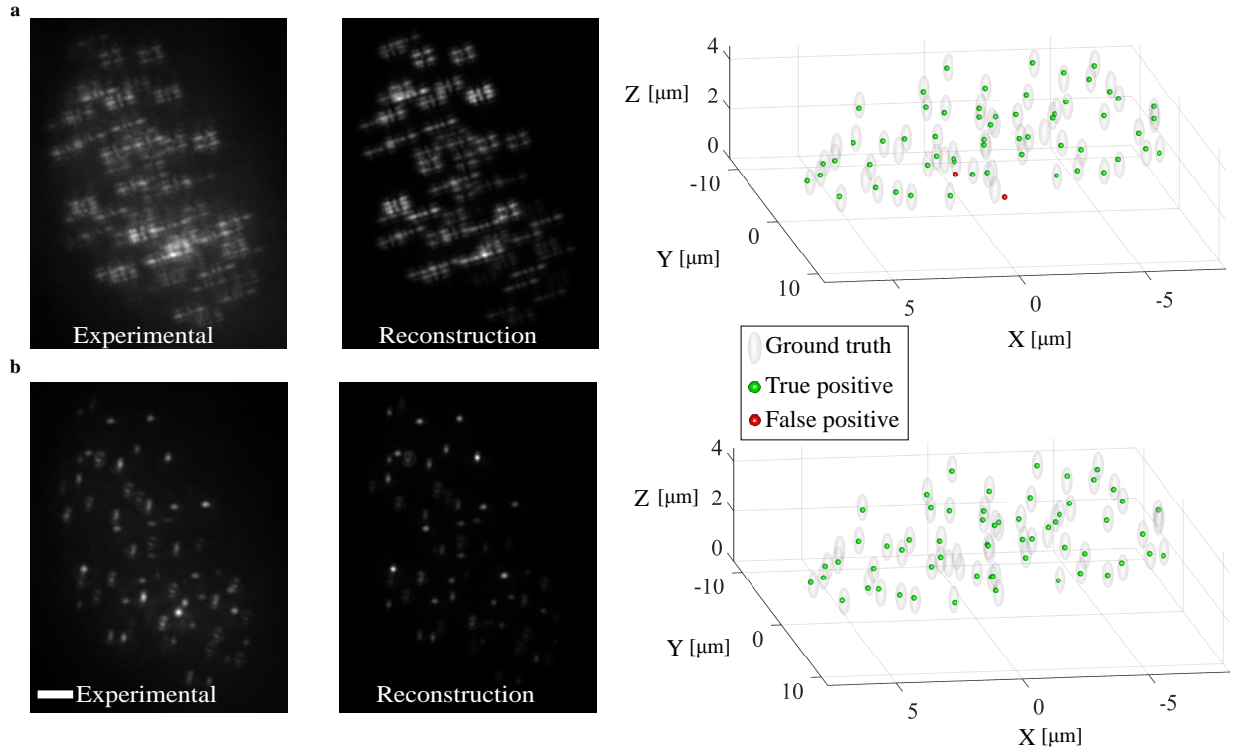

**Fig. S19. Experimental demonstration for a higher focus setting.** **a** Experimental snapshot with the Tetrapod PSF (left), rendered image from the 3D recovered positions by the Tetrapod CNN (middle), and a 3D comparison of the recovered positions and the approximate experimental ground truth (right). **b** Experimental snapshot with the learned PSF (left), rendered image from the 3D recovered positions by the learned PSF CNN (middle), and a 3D comparison of the recovered positions and the approximate experimental ground truth (right). Note that the reconstructions PSFs were scaled according to their retrieved intensity, therefore some appear dim, however their positions are correctly recovered as apparent in the right figures. The Jaccard index for the Tetrapod PSF was 0.85 compared to 0.89 for the learned PSF. Scale bar is 3  $\mu\text{m}$ .

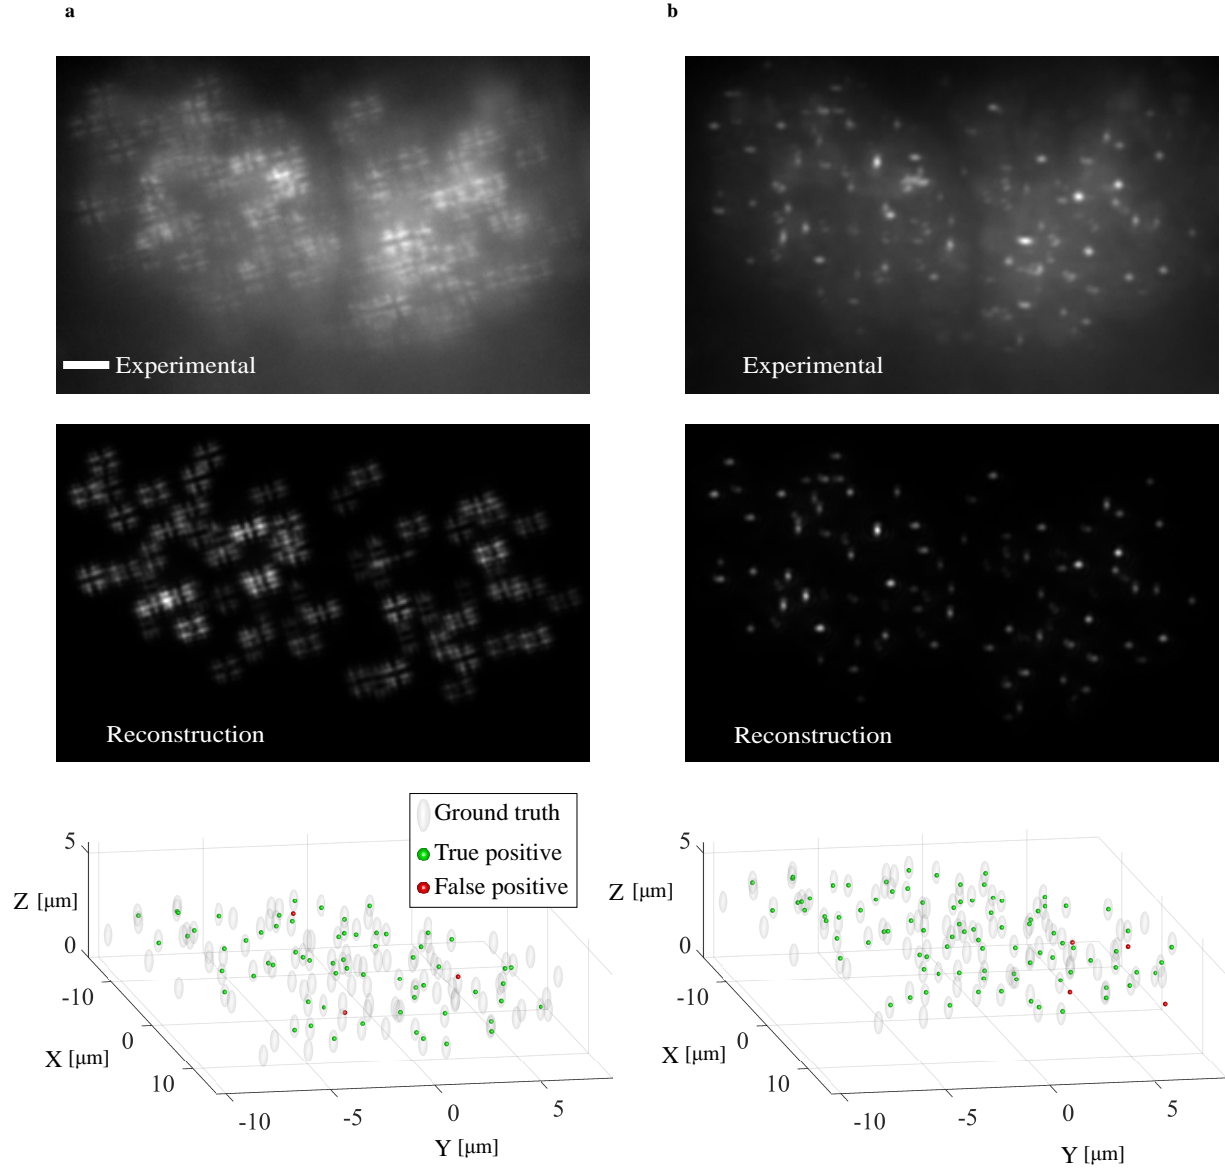

**Fig. S20. Experimental demonstration for a lower SNR.** **a** Experimental snapshot with the Tetrapod PSF (top), rendered image from the 3D recovered positions by the Tetrapod CNN (middle), and a 3D comparison of the recovered positions and the approximate experimental ground truth (bottom). **b** Experimental snapshot with the learned PSF (top), rendered image from the 3D recovered positions by the learned PSF CNN (middle), and a 3D comparison of the recovered positions and the approximate experimental ground truth (bottom). Note that the reconstructions PSFs were scaled according to their retrieved intensity, therefore some appear dim, however their positions are correctly recovered as apparent in the right figures. The Jaccard index for the Tetrapod PSF was 0.52 compared to 0.72 for the learned PSF. Scale bar is 3  $\mu\text{m}$ .

## References

- [1] J. Long, E. Shelhamer, and T. Darrell, "Fully convolutional networks for semantic segmentation," in *Proceedings of the IEEE conference on computer vision and pattern recognition*, pp. 3431–3440, 2015.
- [2] S. Ioffe and C. Szegedy, "Batch normalization: Accelerating deep network training by reducing internal covariate shift," in *Proceedings of the 32nd International Conference on Machine Learning* (F. Bach and D. Blei, eds.), vol. 37 of *Proceedings of Machine Learning Research*, (Lille, France), pp. 448–456, PMLR, 07–09 Jul 2015.
- [3] D. Ulyanov, A. Vedaldi, and V. Lempitsky, "Instance normalization: The missing ingredient for fast stylization," *arXiv preprint arXiv:1607.08022*, 2016.
- [4] F. Yu and V. Koltun, "Multi-scale context aggregation by dilated convolutions," *arXiv preprint arXiv:1511.07122*, 2015.
- [5] K. He, X. Zhang, S. Ren, and J. Sun, "Deep Residual Learning for Image Recognition," *2016 IEEE Conference on Computer Vision and Pattern Recognition (CVPR)*, pp. 770–778, 2016.

- [6] A. Newell, K. Yang, and J. Deng, "Stacked hourglass networks for human pose estimation," in *European Conference on Computer Vision*, pp. 483–499, Springer, 2016.
- [7] G. Pavlakos, X. Zhou, K. G. Derpanis, and K. Daniilidis, "Coarse-to-fine volumetric prediction for single-image 3d human pose," in *Proceedings of the IEEE Conference on Computer Vision and Pattern Recognition*, pp. 7025–7034, 2017.
- [8] A. Odena, V. Dumoulin, and C. Olah, "Deconvolution and checkerboard artifacts," *Distill*, 2016.
- [9] M. D. Zeiler, D. Krishnan, G. W. Taylor, and R. Fergus, "Deconvolutional networks," in *Cvpr*, vol. 10, p. 7, 2010.
- [10] M. D. Zeiler and R. Fergus, "Visualizing and understanding convolutional networks," in *European conference on computer vision*, pp. 818–833, Springer, 2014.
- [11] V. Dumoulin and F. Visin, "A guide to convolution arithmetic for deep learning," *arXiv preprint arXiv:1603.07285*, 2016.
- [12] W. Shi, J. Caballero, F. Huszár, J. Totz, A. P. Aitken, R. Bishop, D. Rueckert, and Z. Wang, "Real-time single image and video super-resolution using an efficient sub-pixel convolutional neural network," in *Proceedings of the IEEE conference on computer vision and pattern recognition*, pp. 1874–1883, 2016.
- [13] A. Aitken, C. Ledig, L. Theis, J. Caballero, Z. Wang, and W. Shi, "Checkerboard artifact free sub-pixel convolution: A note on sub-pixel convolution, resize convolution and convolution resize," *arXiv preprint arXiv:1707.02937*, 2017.
- [14] A. L. Maas, A. Y. Hannun, and A. Y. Ng, "Rectifier nonlinearities improve neural network acoustic models," in *Proc. icml*, vol. 30, p. 3, 2013.
- [15] H. Zhang, Q. Li, and Z. Sun, "Joint voxel and coordinate regression for accurate 3d facial landmark localization," in *2018 24th International Conference on Pattern Recognition (ICPR)*, pp. 2202–2208, IEEE, 2018.
- [16] Y. Shechtman, S. J. Sahl, A. S. Backer, and W. Moerner, "Optimal point spread function design for 3d imaging," *Physical review letters*, vol. 113, no. 13, p. 133902, 2014.
- [17] S. R. P. Pavani, M. A. Thompson, J. S. Biteen, S. J. Lord, N. Liu, R. J. Twieg, R. Piestun, and W. Moerner, "Three-dimensional, single-molecule fluorescence imaging beyond the diffraction limit by using a double-helix point spread function," *Proceedings of the National Academy of Sciences*, vol. 106, no. 9, pp. 2995–2999, 2009.
- [18] H. Haim, S. Elmaleh, R. Giryas, A. M. Bronstein, and E. Marom, "Depth estimation from a single image using deep learned phase coded mask," *IEEE Transactions on Computational Imaging*, vol. 4, no. 3, pp. 298–310, 2018.
- [19] V. Sitzmann, S. Diamond, Y. Peng, X. Dun, S. Boyd, W. Heidrich, F. Heide, and G. Wetzstein, "End-to-end optimization of optics and image processing for achromatic extended depth of field and super-resolution imaging," *ACM Transactions on Graphics (TOG)*, vol. 37, no. 4, p. 114, 2018.
- [20] Y. Wu, V. Boominathan, H. Chen, A. Sankaranarayanan, and A. Veeraraghavan, "Phasecam3d—learning phase masks for passive single view depth estimation,"
- [21] A. S. Backer and W. Moerner, "Extending single-molecule microscopy using optical fourier processing," *The Journal of Physical Chemistry B*, vol. 118, no. 28, pp. 8313–8329, 2014.
- [22] J. W. Goodman, *Introduction to Fourier optics*. Roberts and Company Publishers, 2005.
- [23] S. Liu, E. B. Kromann, W. D. Krueger, J. Bewersdorf, and K. A. Lidke, "Three dimensional single molecule localization using a phase retrieved pupil function," *Optics express*, vol. 21, no. 24, pp. 29462–29487, 2013.
- [24] N. Bourg, C. Mayet, G. Dupuis, T. Barroca, P. Bon, S. Lécart, E. Fort, and S. Lévêque-Fort, "Direct optical nanoscopy with axially localized detection," *Nature Photonics*, vol. 9, no. 9, p. 587, 2015.
- [25] B. Richards and E. Wolf, "Electromagnetic diffraction in optical systems, ii. structure of the image field in an aplanatic system," *Proceedings of the Royal Society of London. Series A. Mathematical and Physical Sciences*, vol. 253, no. 1274, pp. 358–379, 1959.
- [26] N. Boyd, E. Jonas, H. P. Babcock, and B. Recht, "Deeploco: Fast 3d localization microscopy using neural networks," *BioRxiv*, p. 267096, 2018.
- [27] D. Sage, T.-A. Pham, H. Babcock, T. Lukes, T. Pengo, J. Chao, R. Velmurugan, A. Herbert, A. Agrawal, S. Colabrese, *et al.*, "Super-resolution fight club: assessment of 2d and 3d single-molecule localization microscopy software," *Nature methods*, vol. 16, no. 5, p. 387, 2019.
- [28] H. P. Babcock and X. Zhuang, "Analyzing single molecule localization microscopy data using cubic splines," *Scientific reports*, vol. 7, no. 1, p. 552, 2017.
- [29] P. N. Petrov, Y. Shechtman, and W. Moerner, "Measurement-based estimation of global pupil functions in 3d localization microscopy," *Optics express*, vol. 25, no. 7, pp. 7945–7959, 2017.
- [30] A. Aristov, B. Lelandais, E. Rensen, and C. Zimmer, "Zola-3d allows flexible 3d localization microscopy over an adjustable axial range," *Nature communications*, vol. 9, no. 1, p. 2409, 2018.
- [31] M. Hirsch, R. J. Wareham, M. L. Martin-Fernandez, M. P. Hobson, and D. J. Rolfe, "A stochastic model for electron multiplication charge-coupled devices—from theory to practice," *PloS one*, vol. 8, no. 1, p. e53671, 2013.
- [32] F. Huang, T. M. Hartwich, F. E. Rivera-Molina, Y. Lin, W. C. Duim, J. J. Long, P. D. Uchil, J. R. Myers, M. A. Baird, W. Mothes, *et al.*, "Video-rate nanoscopy using sCMOS camera-specific single-molecule localization algorithms," *Nature methods*, vol. 10, no. 7, p. 653, 2013.
- [33] D. P. Kingma and M. Welling, "Auto-encoding variational bayes," *arXiv preprint arXiv:1312.6114*, 2013.
- [34] F. J. Flanagan, *Complex variables: harmonic and analytic functions*. Courier Corporation, 1983.
- [35] R. Remmert, *Theory of complex functions*, vol. 122. Springer Science & Business Media, 2012.
- [36] R. Al-Rfou, G. Alain, A. Almahairi, C. Angermueller, D. Bahdanau, N. Ballas, F. Bastien, J. Bayer, A. Belikov, A. Belopolsky, *et al.*, "Theano: A python framework for fast computation of mathematical expressions," *arXiv preprint arXiv:1605.02688*, 2016.
- [37] K. Kreutz-Delgado, "The complex gradient operator and the cr-calculus," *arXiv preprint arXiv:0906.4835*, 2009.
- [38] A. Paszke, S. Gross, S. Chintala, G. Chanan, E. Yang, Z. DeVito, Z. Lin, A. Desmaison, L. Antiga, and A. Lerer, "Automatic differentiation in pytorch," 2017.

- [39] O. Rippel, J. Snoek, and R. P. Adams, "Spectral representations for convolutional neural networks," in *Advances in neural information processing systems*, pp. 2449–2457, 2015.
- [40] Y. Li, M. Mund, P. Hoess, J. Deschamps, U. Matti, B. Nijmeijer, V. J. Sabinina, J. Ellenberg, I. Schoen, and J. Ries, "Real-time 3d single-molecule localization using experimental point spread functions," *Nature methods*, vol. 15, no. 5, p. 367, 2018.
- [41] M. Born and E. Wolf, *Principles of optics: electromagnetic theory of propagation, interference and diffraction of light*. Elsevier, 2013.
- [42] P. Zelger, K. Kaser, B. Rossboth, L. Velas, G. Schütz, and A. Jesacher, "Three-dimensional localization microscopy using deep learning," *Optics express*, vol. 26, no. 25, pp. 33166–33179, 2018.
- [43] W. Wang, F. Ye, H. Shen, N. A. Moringo, C. Dutta, J. T. Robinson, and C. F. Landes, "Generalized method to design phase masks for 3d super-resolution microscopy," *Optics express*, vol. 27, no. 3, pp. 3799–3816, 2019.
- [44] X. Cao, Y. Wei, F. Wen, and J. Sun, "Face alignment by explicit shape regression," *International Journal of Computer Vision*, vol. 107, no. 2, pp. 177–190, 2014.
- [45] E. Nehme, L. E. Weiss, T. Michaeli, and Y. Shechtman, "Deep-storm: super-resolution single-molecule microscopy by deep learning," *Optica*, vol. 5, no. 4, pp. 458–464, 2018.
- [46] A. Nibali, Z. He, S. Morgan, and L. Prendergast, "Numerical coordinate regression with convolutional neural networks," *arXiv preprint arXiv:1801.07372*, 2018.
- [47] M. Lin, Q. Chen, and S. Yan, "Network in network," *arXiv preprint arXiv:1312.4400*, 2013.
- [48] E. Hershko, L. E. Weiss, T. Michaeli, and Y. Shechtman, "Multicolor localization microscopy and point-spread-function engineering by deep learning," *Optics express*, vol. 27, no. 5, pp. 6158–6183, 2019.
- [49] T.-Y. Lin, P. Goyal, R. Girshick, K. He, and P. Dollár, "Focal loss for dense object detection," in *Proceedings of the IEEE international conference on computer vision*, pp. 2980–2988, 2017.
- [50] N. Zhang, E. Shelhamer, Y. Gao, and T. Darrell, "Fine-grained pose prediction, normalization, and recognition," *arXiv preprint arXiv:1511.07063*, 2015.
- [51] L. Pishchulin, E. Insafutdinov, S. Tang, B. Andres, M. Andriluka, P. V. Gehler, and B. Schiele, "Deepcut: Joint subset partition and labeling for multi person pose estimation," in *Proceedings of the IEEE Conference on Computer Vision and Pattern Recognition*, pp. 4929–4937, 2016.
- [52] E. Insafutdinov, L. Pishchulin, B. Andres, M. Andriluka, and B. Schiele, "Deepcut: A deeper, stronger, and faster multi-person pose estimation model," in *European Conference on Computer Vision*, pp. 34–50, Springer, 2016.
- [53] M. A. Rahman and Y. Wang, "Optimizing intersection-over-union in deep neural networks for image segmentation," in *International symposium on visual computing*, pp. 234–244, Springer, 2016.
- [54] F. Milletari, N. Navab, and S.-A. Ahmadi, "V-net: Fully convolutional neural networks for volumetric medical image segmentation," in *2016 Fourth International Conference on 3D Vision (3DV)*, pp. 565–571, IEEE, 2016.
- [55] R. Lguensat, M. Sun, R. Fablet, P. Tandeo, E. Mason, and G. Chen, "Eddynet: A deep neural network for pixel-wise classification of oceanic eddies," in *IGARSS 2018-2018 IEEE International Geoscience and Remote Sensing Symposium*, pp. 1764–1767, IEEE, 2018.
- [56] M. Berman, A. Rannen Triki, and M. B. Blaschko, "The lovász-softmax loss: A tractable surrogate for the optimization of the intersection-over-union measure in neural networks," in *Proceedings of the IEEE Conference on Computer Vision and Pattern Recognition*, pp. 4413–4421, 2018.
- [57] D. C. Luvizon, H. Tabia, and D. Picard, "Human pose regression by combining indirect part detection and contextual information," *arXiv preprint arXiv:1710.02322*, 2017.
- [58] X. Sun, B. Xiao, F. Wei, S. Liang, and Y. Wei, "Integral human pose regression," in *Proceedings of the European Conference on Computer Vision (ECCV)*, pp. 529–545, 2018.
- [59] D. P. Kingma and J. Ba, "Adam: A method for stochastic optimization," *arXiv preprint arXiv:1412.6980*, 2014.
- [60] Y. Wu and K. He, "Group normalization," in *Proceedings of the European Conference on Computer Vision (ECCV)*, pp. 3–19, 2018.
- [61] I. Loshchilov and F. Hutter, "Decoupled weight decay regularization," 2018.
- [62] L. Wan, M. Zeiler, S. Zhang, Y. Le Cun, and R. Fergus, "Regularization of neural networks using dropconnect," in *International conference on machine learning*, pp. 1058–1066, 2013.
- [63] Y. Shechtman, L. E. Weiss, A. S. Backer, S. J. Sahl, and W. Moerner, "Precise three-dimensional scan-free multiple-particle tracking over large axial ranges with tetrapod point spread functions," *Nano letters*, vol. 15, no. 6, pp. 4194–4199, 2015.
- [64] S. J. Holden, S. Uphoff, and A. N. Kapanidis, "Daostorm: an algorithm for high-density super-resolution microscopy," *Nature methods*, vol. 8, no. 4, p. 279, 2011.
- [65] F. Huang, S. L. Schwartz, J. M. Byars, and K. A. Lidke, "Simultaneous multiple-emitter fitting for single molecule super-resolution imaging," *Biomedical optics express*, vol. 2, no. 5, pp. 1377–1393, 2011.
- [66] H. Babcock, Y. M. Sigal, and X. Zhuang, "A high-density 3d localization algorithm for stochastic optical reconstruction microscopy," *Optical Nanoscopy*, vol. 1, no. 1, p. 6, 2012.
- [67] S. M. Kay, *Fundamentals of statistical signal processing*. Prentice Hall PTR, 1993.
- [68] A. V. Abraham, S. Ram, J. Chao, E. Ward, and R. J. Ober, "Quantitative study of single molecule location estimation techniques," *Optics express*, vol. 17, no. 26, pp. 23352–23373, 2009.
- [69] S. G. Mallat and Z. Zhang, "Matching pursuits with time-frequency dictionaries," *IEEE Transactions on signal processing*, vol. 41, no. 12, pp. 3397–3415, 1993.
- [70] Y. C. Pati, R. Rezaifar, and P. S. Krishnaprasad, "Orthogonal matching pursuit: Recursive function approximation with applications to wavelet decomposition," in *Proceedings of 27th Asilomar conference on signals, systems and computers*, pp. 40–44, IEEE, 1993.
- [71] P. Zhang, S. Liu, A. Chaurasia, D. Ma, M. J. Mlodzianoski, E. Culurciello, and F. Huang, "Analyzing complex single-molecule emission patterns with deep learning," *Nature methods*, vol. 15, no. 11, p. 913, 2018.

- [72] H. W. Kuhn, "The hungarian method for the assignment problem," *Naval research logistics quarterly*, vol. 2, no. 1-2, pp. 83–97, 1955.
- [73] L. Carlini, S. J. Holden, K. M. Douglass, and S. Manley, "Correction of a depth-dependent lateral distortion in 3d super-resolution imaging," *PLoS One*, vol. 10, no. 11, p. e0142949, 2015.
- [74] M. Ovesný, P. Křížek, J. Borkovec, Z. Švindrych, and G. M. Hagen, "Thunderstorm: a comprehensive imagej plug-in for palm and storm data analysis and super-resolution imaging," *Bioinformatics*, vol. 30, no. 16, pp. 2389–2390, 2014.
- [75] S. Hell, G. Reiner, C. Cremer, and E. H. Stelzer, "Aberrations in confocal fluorescence microscopy induced by mismatches in refractive index," *Journal of microscopy*, vol. 169, no. 3, pp. 391–405, 1993.
- [76] B. Huang, W. Wang, M. Bates, and X. Zhuang, "Three-dimensional super-resolution imaging by stochastic optical reconstruction microscopy," *Science*, vol. 319, no. 5864, pp. 810–813, 2008.
